# Supplementary material for: A Unified Framework for Long Range and Cold Start Forecasting of Seasonal Profiles in Time Series
Source: arXiv:1710.08473 source file (2018-08-26)
Supplement: Supplementary file 1 [file appendix.tex]

%\section{Appendix}
%\label{sec:appendix}

\section{Experiment Details}
\label{appendix:experiment_details}

\paragraph{Cross validation}
For each forecasting experiment, we separately run 5-fold cross validation over a grid in order to select the model hyperparameters. Because some of our loss functions are nonconvex, this requires running random restarts. Since this is computationally expensive, we perform an approximation to full grid search. We perform a two-stage cross validation where we first run standard 5-fold cross validation over the hyperparameters in the non-matrix factorization models. The regularization parameters for these models are a subset of the respective corresponding model that includes matrix factorization, so we then fix those hyperparameter values in the corresponding models with matrix factorization and cross validate over the remaining hyperparameters. Looking at Eq. (4) in the main paper, we would first cross validate over $\lambda_1$ and fix the selected value while cross validating over $\lambda_2$.

\removed{
\begin{figure*}[t!]
\begin{center}

\begin{subfigure}[t]{0.31\linewidth}
\includegraphics[width=\linewidth, height=3cm]{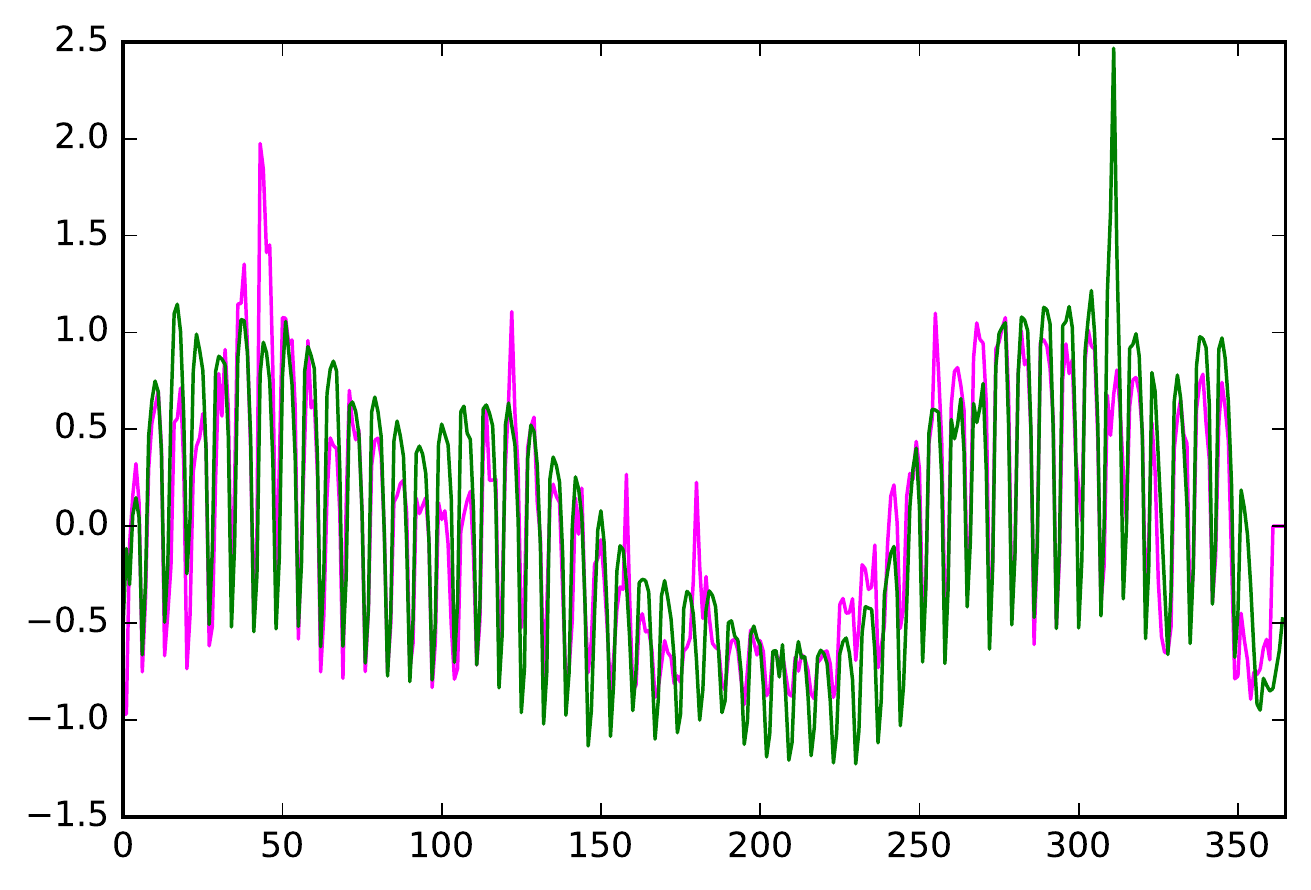}
\vspace{-.5cm}
\caption{James Madison 2014}
\label{fig:ex_longrange_a}
\end{subfigure}
\hfill
\begin{subfigure}[t]{0.31\linewidth}
\includegraphics[width=\linewidth, height=3cm]{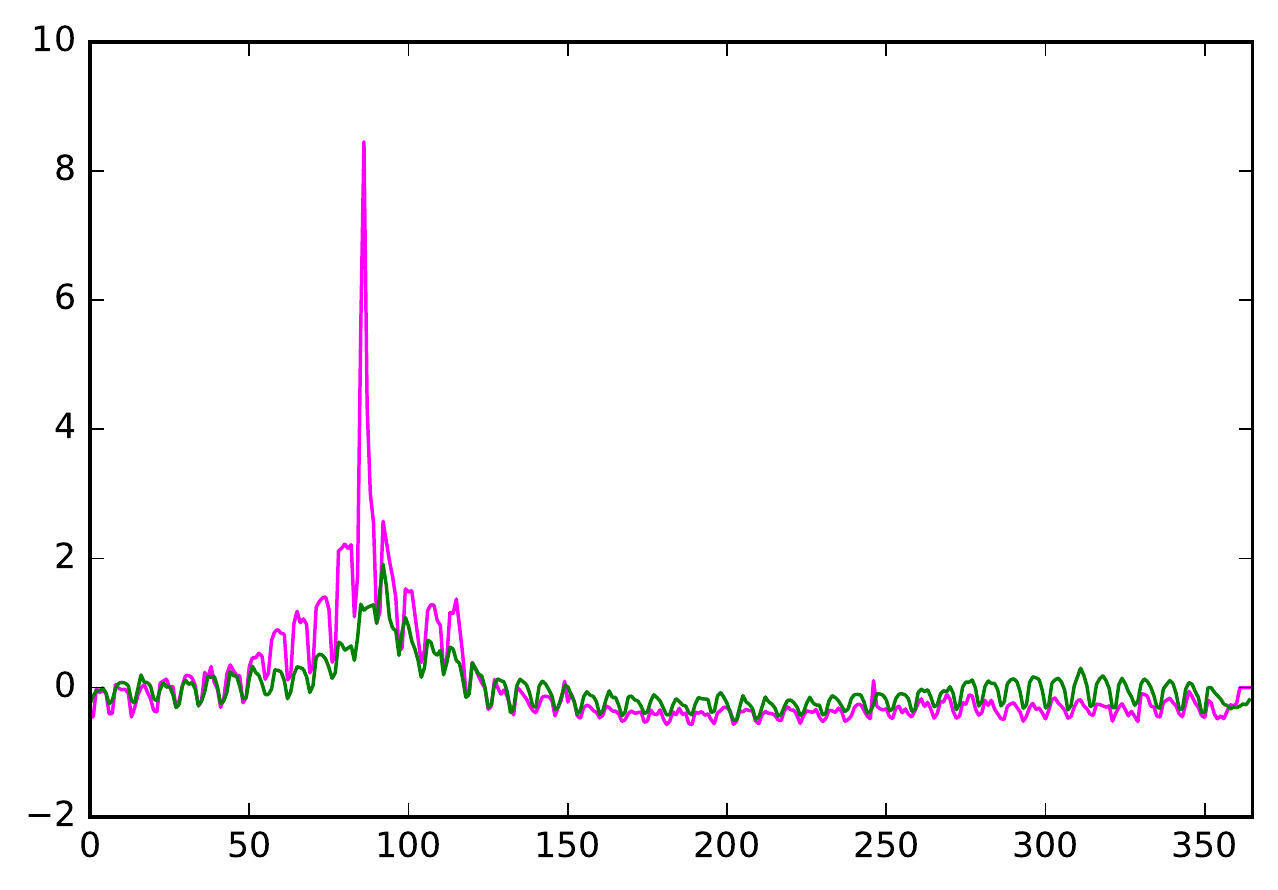}
\vspace{-.5cm}
\caption{April 2014}
\label{fig:ex_longrange_d}
\end{subfigure}
\hfill
\begin{subfigure}[t]{0.31\textwidth}
\includegraphics[width=\linewidth, height=3cm]{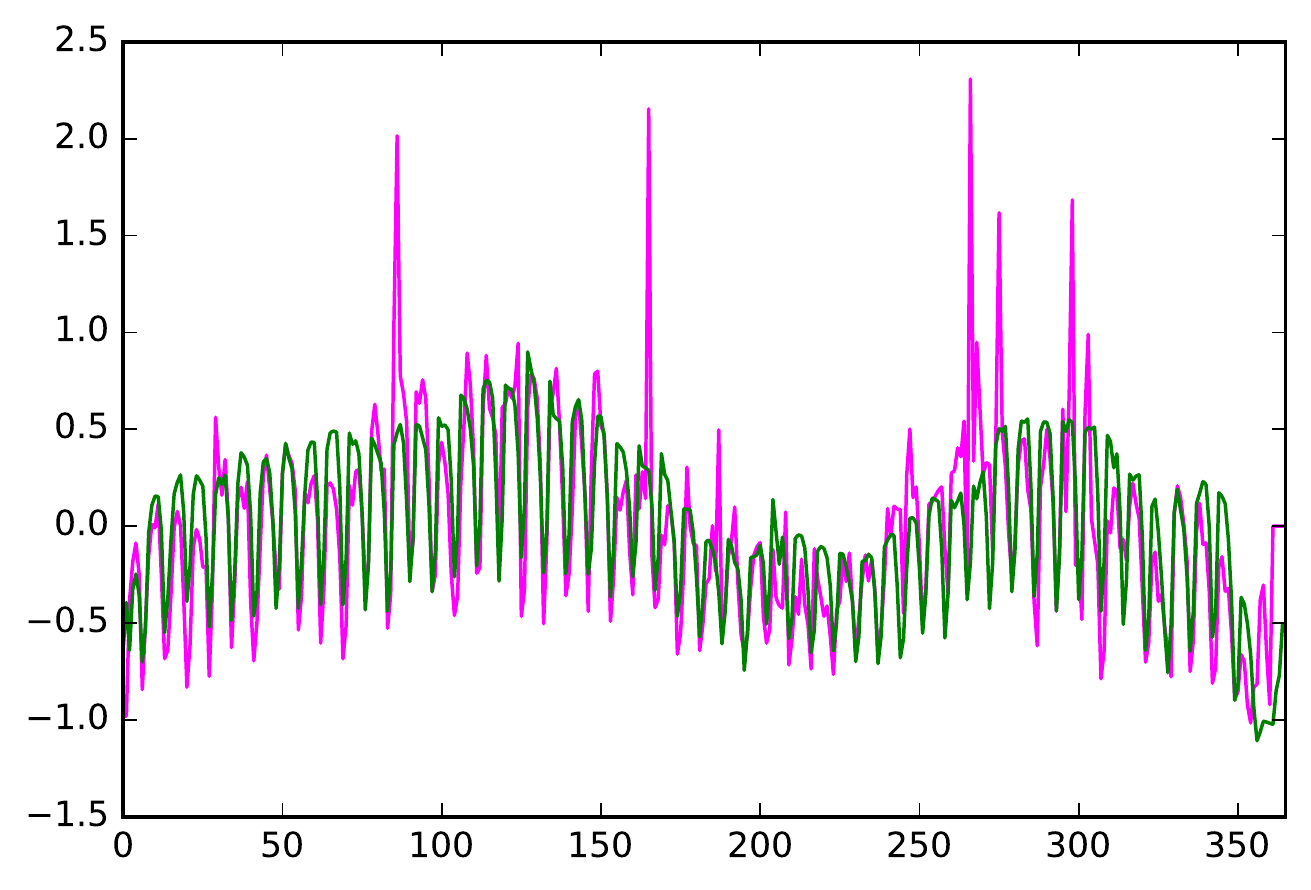}
\vspace{-.5cm}
\caption{Baseball 2014} 
\label{fig:ex_longrange_h}
\end{subfigure}

\medskip
\vspace{-.2cm}

\begin{subfigure}[t]{0.31\linewidth}
\includegraphics[width=\linewidth, height=3cm]{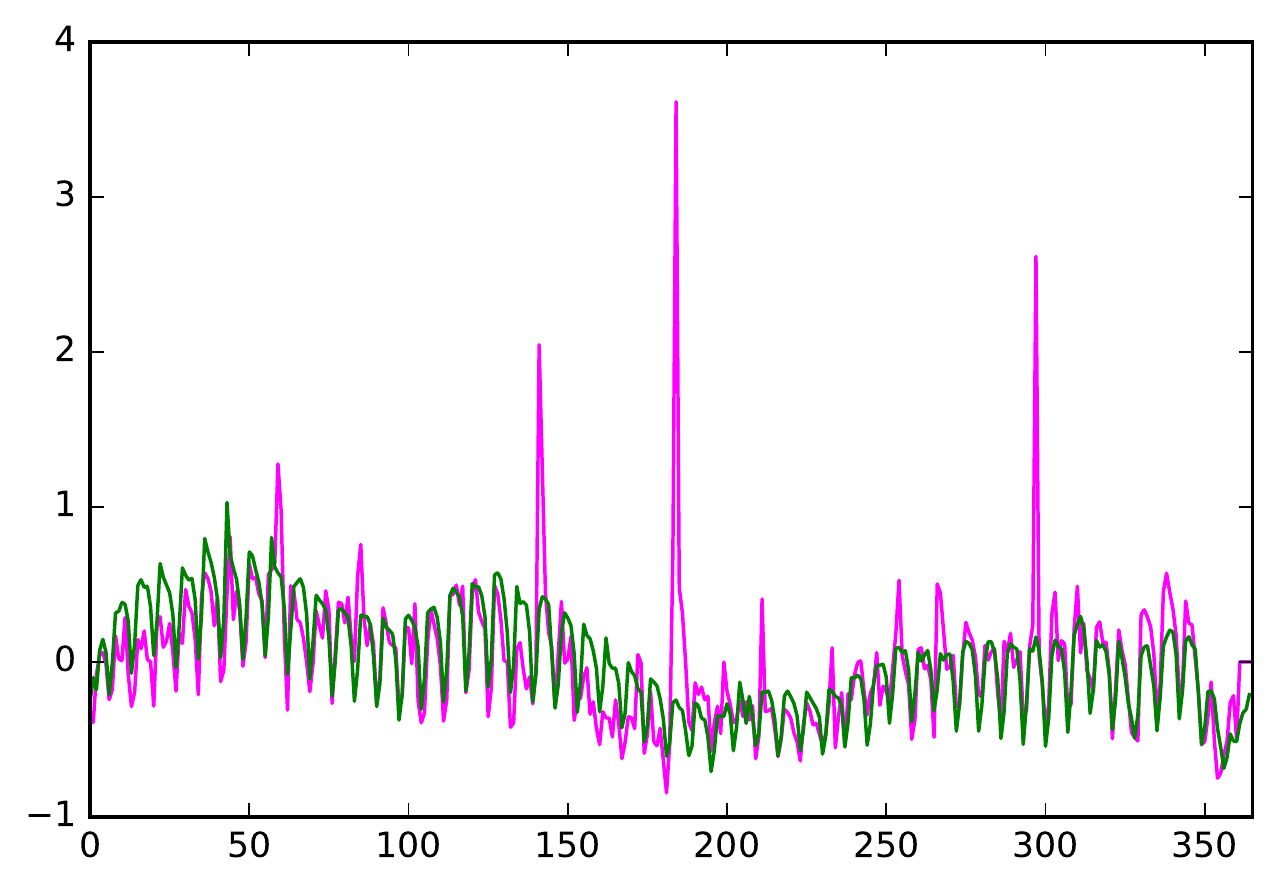}
\vspace{-.5cm}
\caption{Miles Davis 2014}
\label{fig:ex_cs_b}
\end{subfigure}
\hfill
\begin{subfigure}[t]{0.31\textwidth}
\includegraphics[width=\linewidth, height=3cm]{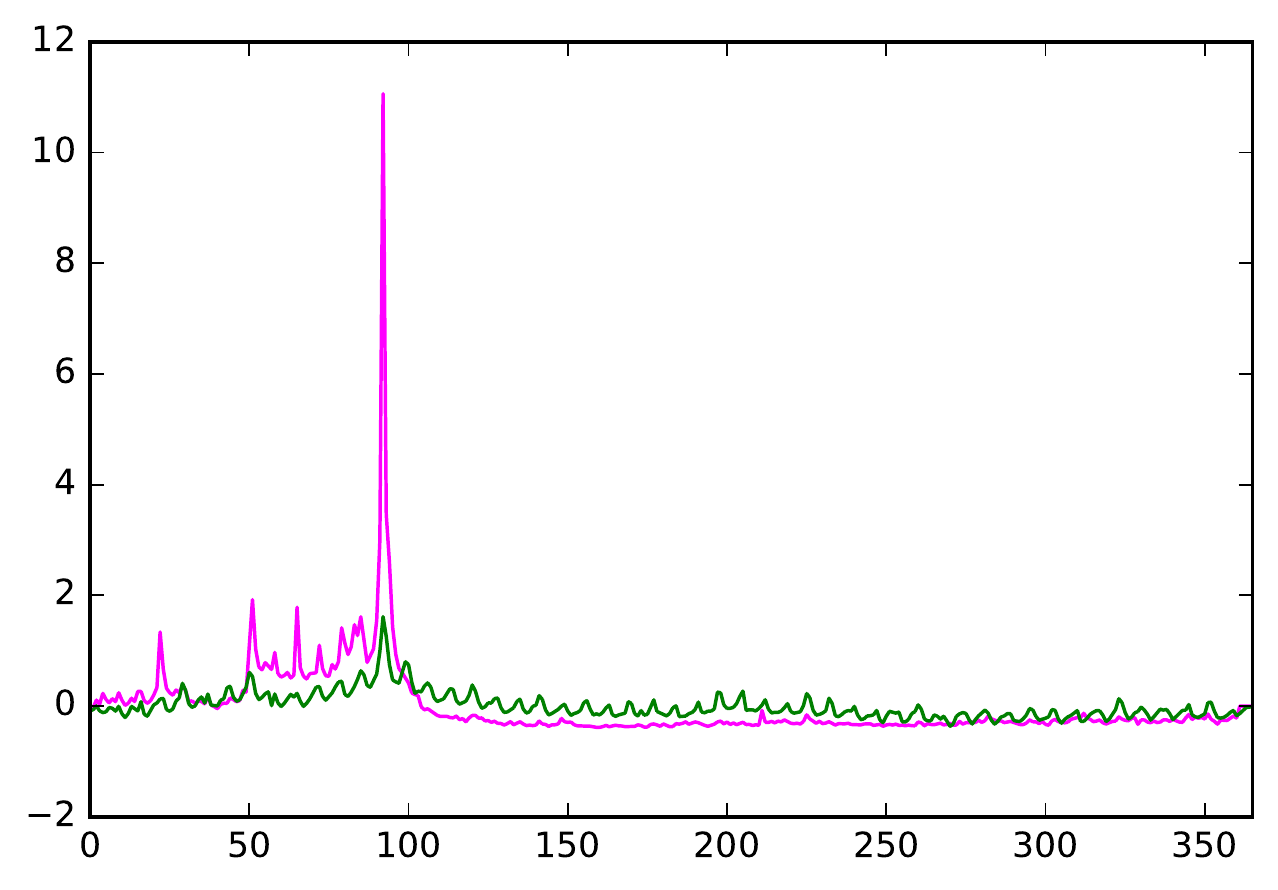}
\vspace{-.5cm}
\caption{WrestleMania 2014} 
\label{fig:ex_cs_h}
\end{subfigure}
\hfill
\begin{subfigure}[t]{0.31\textwidth}
\includegraphics[width=\linewidth, height=3cm]{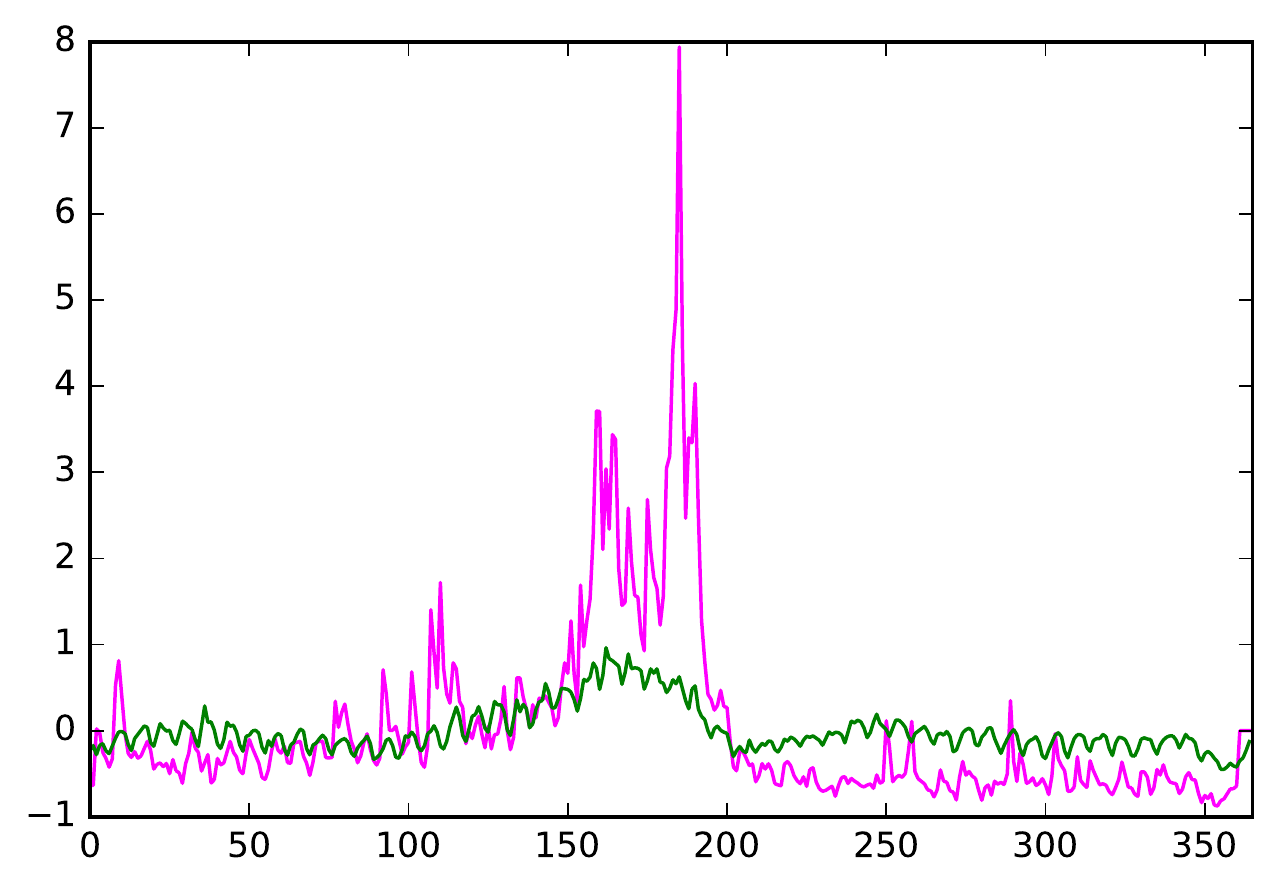}
\vspace{-.5cm}
\caption{Johan Cruyff 2014} 
\label{fig:ex_cs_i}
\end{subfigure}

\vspace{-.2cm}
\caption{Additional predictions of the low-rank plus \texttt{MF} model on the \texttt{Wiki} dataset for long-range (top) and cold-start (bottom) challenges. For the long-range challenge, we show the common yearly structure as discussed in Section \ref{subsec:qualitative_analysis} for \texttt{James Madison}. We capture an increase in predicted page traffic for \texttt{April} around the right time of year. Lastly, for \texttt{Baseball}, we accurately capture this seasonal pattern. For the cold-start challenge, we again show the common yearly structure for \texttt{Miles Davis}. For \texttt{WrestleMania} and \texttt{Johan Cruyff}, our model correctly predicts the location of an annually recurring surge in page traffic despite not having previously
observed any of the series. However, it struggles to capture the magnitude. Both of these articles correspond to a popular sporting events: wrestling for WrestleMania, and the World Cup (soccer) for Johan Cruyff. }
\end{center}
\end{figure*}
}

\subsection{Dataset Collection Details}

\subsubsection{Google Flu Trends}
The Flu Trends dataset consists of weekly estimates of influenza rates in 311 worldwide regions \cite{ginsberg2009detecting}. We scraped all of the data on the existing webpage, resulting in a matrix of 311 time series of weekly influenza rate estimates ($T=52$). For each time series, we zero-mean the data and divide by the standard deviation to standardize the scale. After reorganizing the matrix as described in Section 3, there are 3197 observed years of data. For metadata, we scraped the summary of the relevant Wikipedia page for each region. We removed stopwords, performed tokenization using the Stanford CoreNLP toolkit \cite{manning-EtAl:2014:P14-5}, and calculated TF-IDF representations of these summaries to use as our metadata vectors. Additionally, each word used in our feature vector must be present in at least two articles.  
%We also included latitude and longitude coordinates of each region if available.
After preprocessing, the dimension of the feature vector is $m = 3356$. This matrix is sparse with roughly $2.9\%$ nonzero entries.

\subsubsection{Wikipedia Page Traffic Dataset}
For the Wikipedia dataset, we collected daily page traffic counts from 4031 Wikipedia articles from the beginning of 2008 to the end of 2014 by querying Wiki Trends \cite{wikitrends}. The pages were selected by obtaining a list of the 5000 most popular pages of a given week in March 2016. 
We employ the method of \cite{cleveland1990stl} to detrend the time series data. For each time series, we zero-mean the data and divide by the standard deviation. For each article, we have anywhere between 1 to 7 years of page traffic counts starting from 2008 to 2014. After reorganizing the time series data matrix as described in Section 3 in the main paper, the total number of columns of $Y$ is $N = 29093$. Each year of article traffic has $T = 365$ days.   Furthermore, we shifted each year to start on the first Sunday and padded with zeros. We scraped the summary of the corresponding Wikipedia page, removed stopwords, performed tokenization using the Stanford CoreNLP toolkit \cite{manning-EtAl:2014:P14-5}, and calculated TF-IDF representations of these summaries to use as our metadata vectors. Additionally, each word used in our feature vector must be present in at least two articles. After preprocessing, the dimension of the features is $m = 22193$. This matrix is extremely sparse with roughly $0.5\%$ nonzero entries.

\subsection{Real Data Experiment Details}

\removed{
\paragraph{Test set selection} 
\begin{itemize}
\item[P1)] \textbf{Long-Range Forecasting}: We included the last year of page traffic for each article in the test set. We further removed 20\% of values from the training data to demonstrate the efficacy of our prediction methods in the presence of missing data.

\item[P2)] \textbf{Missing Data}: For each time series, we pick a time point uniformly from the year for the starting point of the missing chunk, and sample a geometric random variable with mean $\frac{T}{2}$ that determines the length of the missing chunk.

\item[P3)] \textbf{Cold-Start Forecasting}: We randomly selected 25\% of the articles and included the last year of page traffic in the test set. We did not include any previous years of such articles from the training set. We further removed 20\% of values from the training data to demonstrate the efficacy of our prediction methods in the presence of missing data.

\end{itemize}
}

\paragraph{Neural network architecture} For the neural network regression, we use a two hidden layer network with ReLU activations. The first hidden layer has 100 nodes and the second hidden layer has $T = 365$ nodes. Finally, the output layer is a regression layer (uses the identity function as the activation function). For simplicity we also do not regularize the weights of the neural network.

\paragraph{Model training: Google Flu} We set $k = k' = 5$ and train the models with minibatch stochastic gradient descent (SGD). We use a minibatch size of 300 and 30,000 iterations. We individually tuned constant step sizes for each model, although they all turned out to be close to 1e-2.  We use 5-fold cross validation to select hyperparameters. For both $\lambda_1$ and $\lambda_2$, we select them from 10 values evenly spread on a log scale from 0.1 to 1000. For the functional regression models, we choose the number of (evenly spaced) knots $K$ from 4, 8, ..., 20. After selecting hyperparameters, we trained each final model with 50,000 iterations and 10 random restarts. We use a validation set to tune the number of epochs the neural network regression models need.

\paragraph{Model training: Wikipedia Page Traffic} We set $k = k' = 20$ and train the models with minibatch SGD. We use a minibatch size of 500 and 10,000 iterations. We individually tuned constant step sizes for each model, although they all turned out to be close to 1e-1 (with the exception that the neural network regression models used a step size of 1e-2). In this setting, since our data is large enough, we use a single validation set to select our hyperparameters as opposed to cross validation. For both $\lambda_1$ and $\lambda_2$, we select them from 10 values evenly spread on a log scale from 0.01 to 1000. We choose the number of (evenly spaced) knots $K$ from $10, 20, \ldots, 100$. After selecting hyperparameters, we trained each final model with 20,000 iterations and 10 random restarts. We use a validation set to tune the number of epochs the neural network regression models need.

\paragraph{Baselines} For TRMF \cite{Yu2015highdim}, we fix latent dimension ($k$ in our framework) to be the same as what we set for our framework (5 for Google Flu, 20 for the Wikipedia dataset). For both TRMF and the AR baseline, we use a lag set of $\{ 1, \ldots, 5 \} \cup \{ 51, 52, 53 \}$ for the Google Flu data, and a lag set of $\{ 1, \ldots, 10 \} \cup \{ 63, \ldots, 70 \} \cup \{ 363, 364, 365, 366\}$. The chosen lag sets allow for the step-ahead models to learn seasonal yearly patterns. For TRMF, we run rolling cross validation to select hyperparameters, using the code provided by \cite{Yu2015highdim}, while for AR, we simply perform maximum likelihood under Gaussian errors. For \texttt{MF} alone, we run cross validation to select the hyperparameters for regularization. For the \texttt{$k$-NN} baseline, we compared $k = 5, 10, 15, 20$ and selected $k = 10$ due to best performance.

\removed{
\section{Synthetic Experiments}

\begin{figure*}[t]
\begin{center}

\begin{subfigure}[t]{0.31\linewidth}
\includegraphics[width=\linewidth, height=3.5cm]{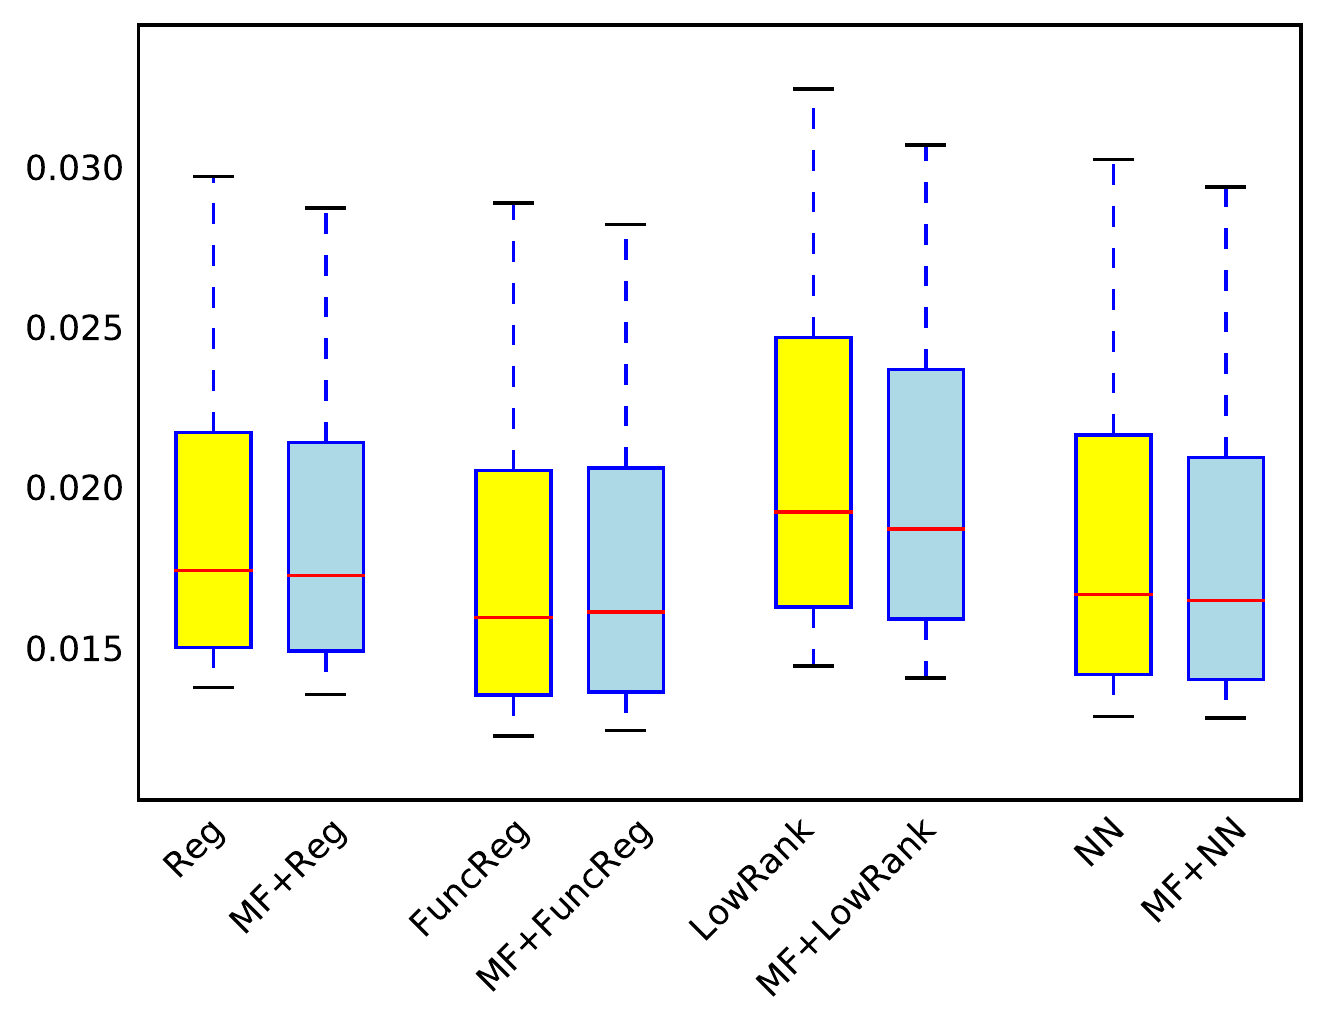}
\caption{Long range}
\label{fig:synth_data_a}
\end{subfigure}
\hfill
\begin{subfigure}[t]{0.31\linewidth}
\includegraphics[width=\linewidth, height=3.5cm]{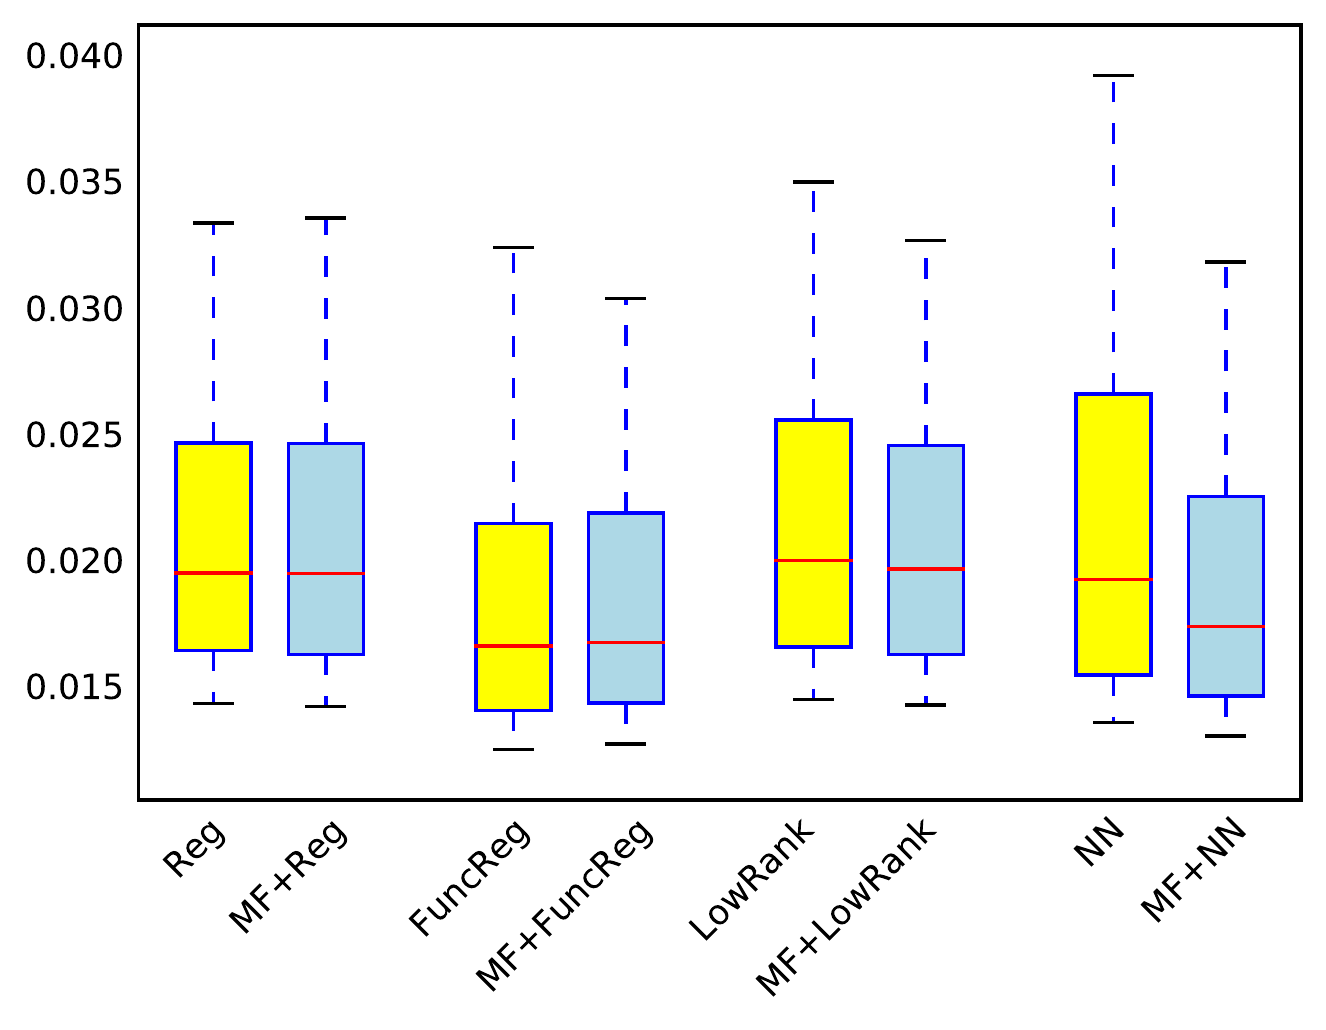}
\caption{Cold-start}
\label{fig:synth_data_b}
\end{subfigure}
\hfill
\begin{subfigure}[t]{0.31\linewidth}
\includegraphics[width=\linewidth, height=3.5cm]{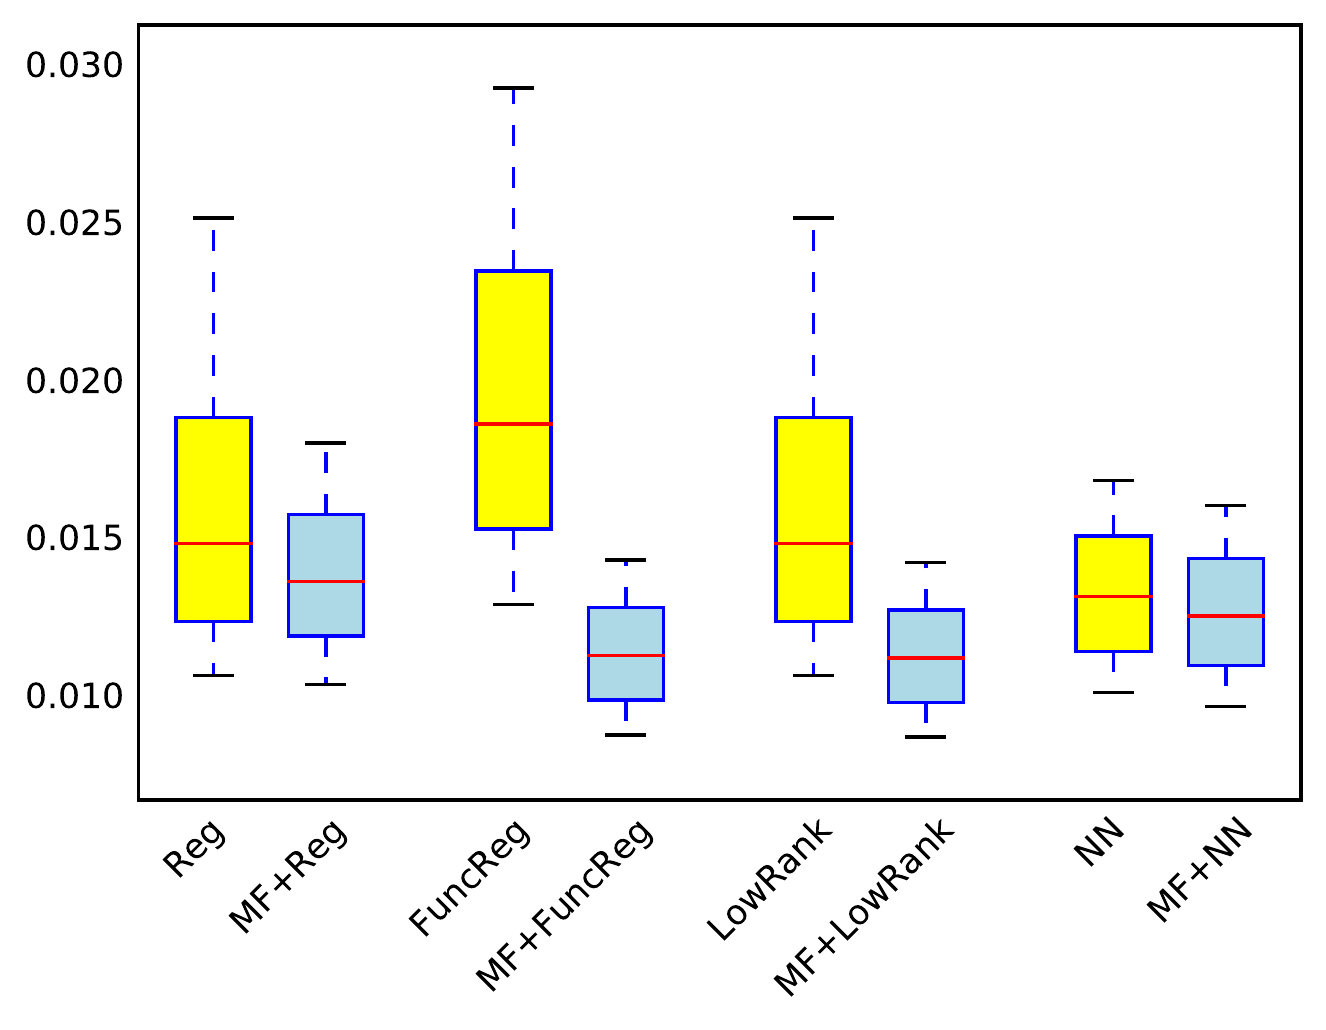}
\caption{Missing data}
\label{fig:synth_data_c}
\end{subfigure}

\caption{Mean Squared Error for long range, cold-start, and missing data experiments on synthetic data.}
\label{fig:synth_data_boxplots}
\end{center}
\end{figure*}

We run experiments showing that when the data exhibits temporal regularity in the form of smoothness, the functional regression models of our framework become very useful.

\paragraph{Synthetic data generation}
We generated data according to the matrix factorization + functional regression model. However, instead of using a B-spline basis for $B$, we sampled each column of $B \in \R^{T \times 50}$ from a smooth Gaussian process with zero mean and double exponential kernel. We sample each column of $L$ as a sine wave with a random period, $Q \sim N\left(0, 0.02 I\right)$, $R_i \sim N\left(0, 0.015 I\right)$, $\veps_i \sim N\left(0, .01 I\right)$, and $\phi_{ik} \sim (1 - z_{ik}) \delta_0 + z_{ik}\text{Exp}(5)$ where $z_{ik} \sim \text{Bernoilli}(.02)$; this is the spike and slab exponential distribution for $\phi_{ik}$ to emulate high-dimensional features that are sparse and positive, e.g. bag-of-words features. We generated a synthetic dataset with dimensions $T = 300, N = 5000, m = 1000, k' = 20$. 

\paragraph{Neural network architecture} For the neural network regression, we use a two hidden layer network with ReLU activations. The first hidden layer has 100 nodes and the second hidden layer has $T = 300$ nodes. Finally, the output layer is a regression layer (uses the identity function as the activation function).

\paragraph{Model training} We run the models with $k = k' = 20$ and train the models with minibatch SGD. We use a minibatch size of 300 and 5,000 iterations. We use a constant step size of 1.0 for the pure regression and low-rank regression models, 0.5 for the functional regression models, and 0.05 for the neural network models. For both $\lambda_1$ and $\lambda_2$, we cross validate over a log scale of 10 values from 0.0001 to 100. To choose the number of (evenly spaced) knots $K$ in the functional regression models, we cross validate over 10, 20, ..., 100. After selecting hyperparameters, we trained each final model with 50,000 iterations and 10 random restarts to avoid local minima. Recall that the neural network models don't have any hyperparameters; We use a validation set to tune the number of epochs the neural network regression models need.

\paragraph{Results} We show quantile box-and-whisker plots of MSE per time series in order to show the distribution of errors in Figure \ref{fig:synth_data_boxplots}. The box encapsulates the 1st to 3rd quartiles, and the whiskers encapsulate the 10th to 90th quantile. Yellow indicates models without MF, and light blue indicates models with MF.

The functional regression models tend to outperform the other models across all prediction challenges as it captures the smoothness of the regression weights across time. The neural network models do not perform as well as the functional regression models, perhaps due to the neural network model not leveraging the smoothness of the series. Adding the matrix factorization component tends to lower high tail error quantiles in  most cases, even in the flexible neural network case. As far as we know, such a structure for neural networks has not been explored. The matrix factorization term captures low-rank structure in the residuals, which results in improved learning of the regression component. 
%Of additional note is that adding the matrix factorization term improves performance in the cold-start (P1) and long-range (P3) challenges, where predictions are only based on the learned regression components and metadata. 
The matrix factorization term also clearly aids performance in the missing data setting (P2).

\section{Two-stage comparison}

In this section, we show an empirical example of where a two-stage approach of 1) imputing missing data via matrix factorization and then 2) learning a regression component on the imputed data leads to weaker prediction results. 

\paragraph{Setup} We generate data the same way as described in the synthetic experiments (Section 4 in this Supplement). To generate missing data, we generate large contiguous chunks of missing data exactly as described in the experiments section of the main paper (Section 4 in the main paper). This type of structure missingness hides the low-rank nature of the data matrix quite well, making it hard for MF to do a good job of imputing the missing values.

\paragraph{Learning} To perform the two-stage approach, we first perform matrix factorization on the training data (which has missing data). Using the learned low-dimensional representation, we impute the missing data to get a fully observed matrix $\hat{Y}$. We then learn a functional regression model (without MF, as shown in Table 1 in the main paper) on $\hat{Y}$, and use this functional regression model to perform long-range and cold-start forecasts. We compare this to our jointly learned MF + functional regression model as shown in Table 1 (of the main paper). 

\paragraph{Results} We show boxplots results in Figure \ref{fig:two_stage_comparison} for all three prediction challenges. We first note that our joint learning approach results in improved performance across all quantiles compared to the two-stage approach. Importantly, the missingness structure makes it difficult for matrix factorization to impute missing values correctly. This leads to learning a regression component on noisy values. Our jointly learned model is able to robustly avoid this issue and provide more accurate forecasts. In the missing data challenge (P2), we see the largest increase in prediction accuracy.

\begin{figure*}[t]
\begin{center}
\includegraphics[scale=0.5]{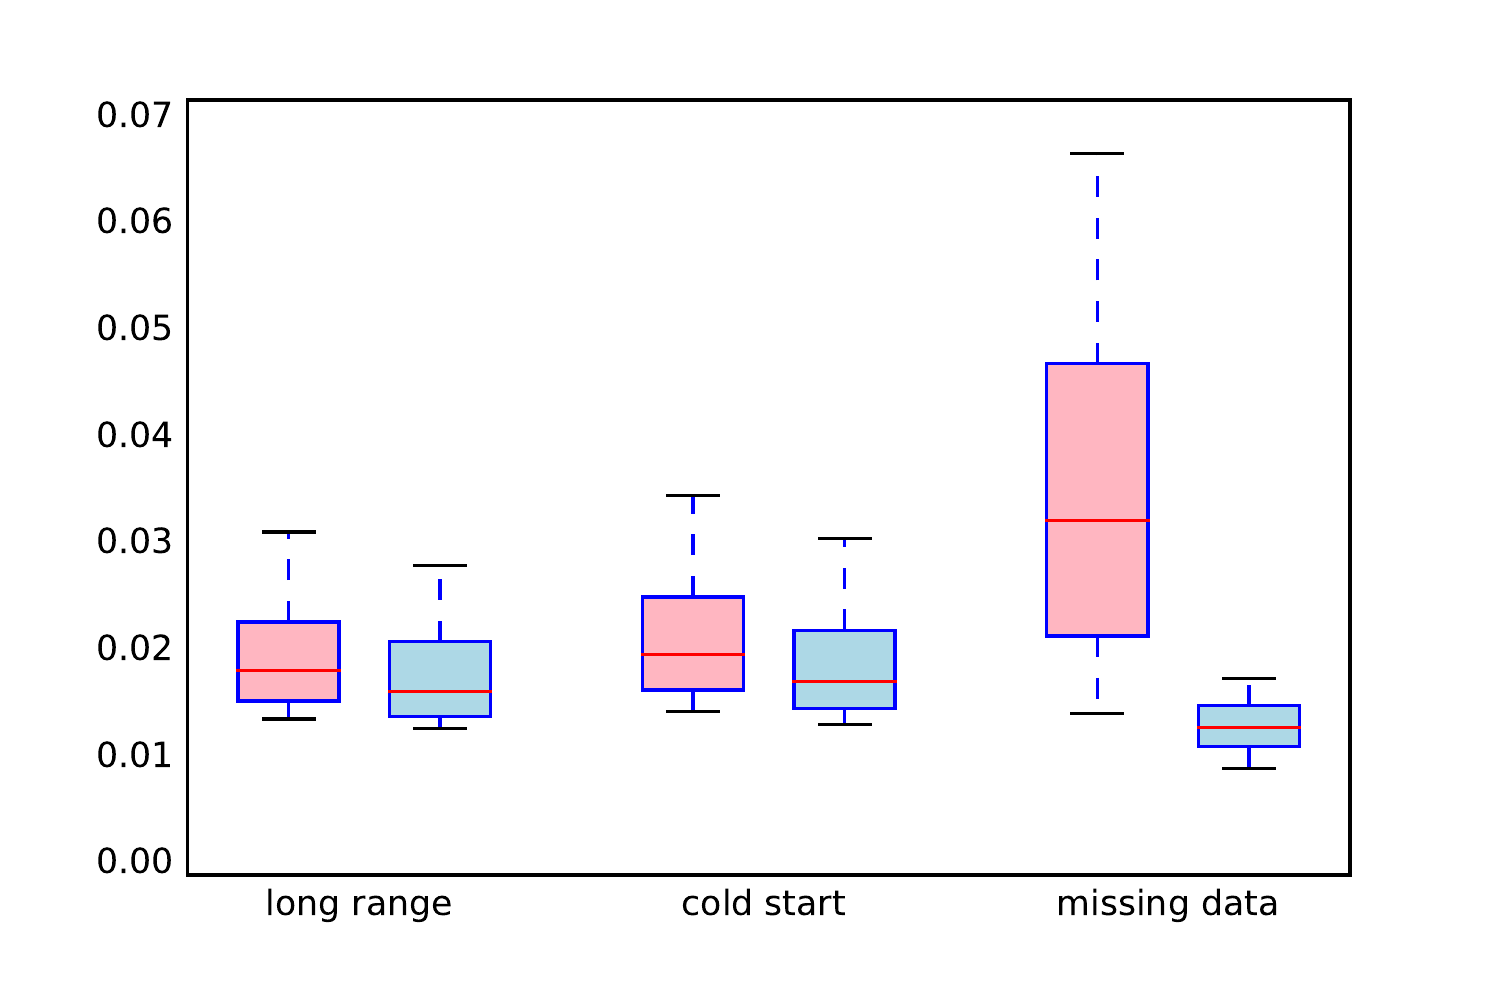}
\caption{Results for the two-stage comparison in mean squared error (MSE) boxplots. In red, we have results for the two-stage approach. In blue, we have results for the jointly learned MF + functional regression model }
\label{fig:two_stage_comparison}
\end{center}
\end{figure*}

\section{Plots}

In this section, we show many more plots to qualitatively evaluate the successes and failures of our matrix factorization + low-rank regression model, which we observed to be most consistently successful across all three forecasting challenges on both the Google flu and Wikipedia data sets. In Figures \ref{fig:mflrr_longrange_example_predictions} and \ref{fig:mflrr_coldstart_example_predictions}, we plot example predictions from the MF + low-rank model on Wikipedia test series for the long-range and cold-start challenges, respectively. We aim to illustrate both the challenge of prediction on complex real-world data and the variety of seasonal profiles that our method is able to forecast.

In Figure \ref{fig:best_trmf_predictions}, we show a comparison between TRMF and MF + low-rank in terms of long-range Wikipedia predictions. We plot the five series closest to the $10^{th}$ quantile of mdAPE for TRMF, thus selecting a set of examples that we know \emph{a priori} to be very favorable for this method. Nonetheless, the results show that our MF + low-rank approach is generally able to produce forecasts with superior prediction of seasonal and oscillatory behavior, even on the test series where TRMF performs close to its best. In this figure, TRMF \textcolor{blue}{predictions} are plotted in blue.

Lastly, to give a sense of the distribution of MF + low-rank prediction quality over the Wikipedia long-range test set, we plot the three series closest to each of the $10^{th}$, $50^{th}$, and $90^{th}$ quantiles of mdAPE error in Figure \ref{fig:mflrr_quantile_examples}. For all figures, recall that the \textcolor{magenta}{observed time series} is in magenta and \textcolor{ForestGreen}{predictions} are overlayed in green. 

} % ending of \removed{ which is before Synthetic Experiments section

\removed{
\begin{figure*}[t!]
\begin{center}

\begin{subfigure}[t]{0.31\linewidth}
\includegraphics[width=\linewidth, height=3cm]{images/example_preds/example_oos_0.pdf}
\vspace{-.5cm}
\caption{James Madison 2014}
\label{fig:ex_longrange_a}
\end{subfigure}
\hfill
\begin{subfigure}[t]{0.31\linewidth}
\includegraphics[width=\linewidth, height=3cm]{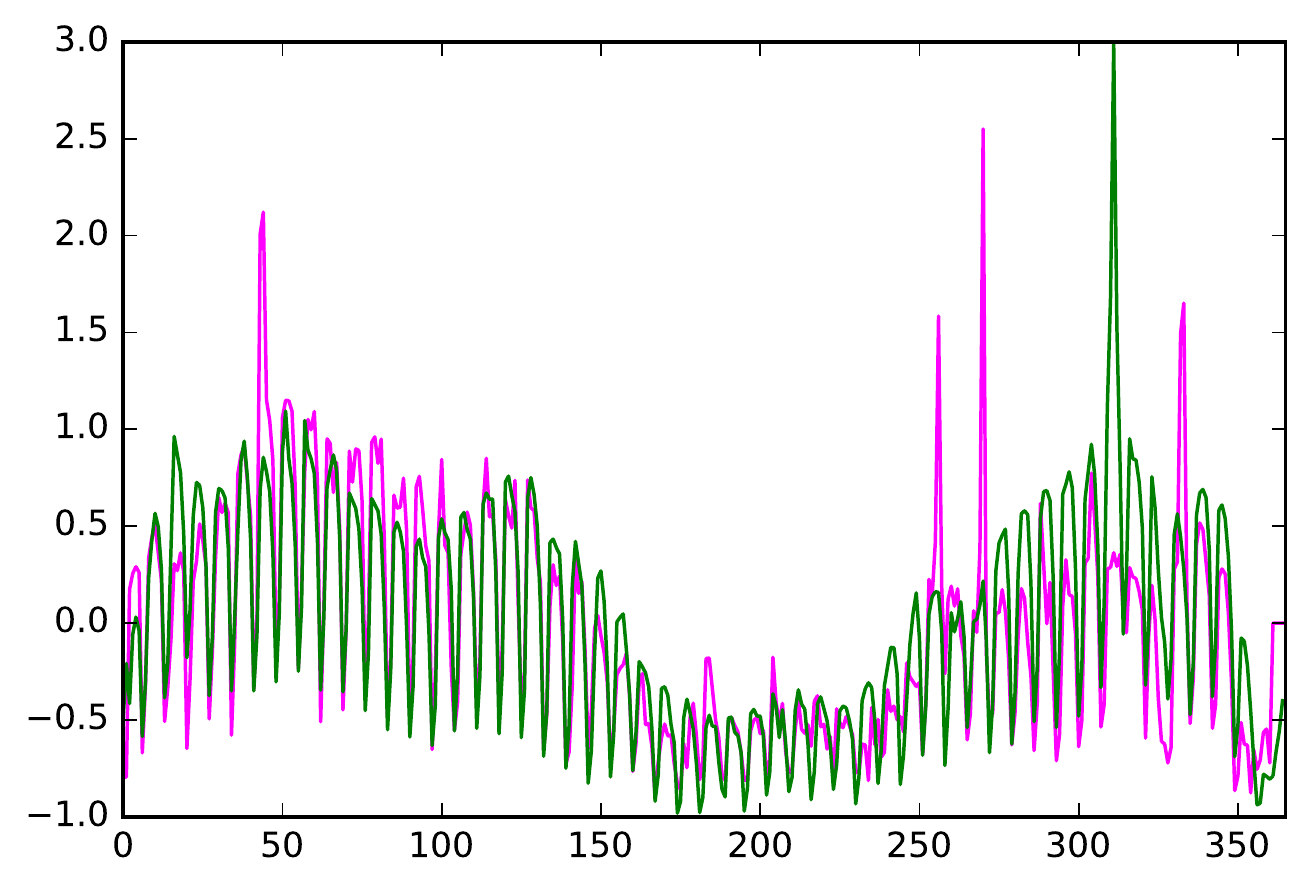}
\vspace{-.5cm}
\caption{Herbert Hoover 2014}
\label{fig:ex_longrange_b}
\end{subfigure}
\hfill
\begin{subfigure}[t]{0.31\textwidth}
\includegraphics[width=\linewidth, height=3cm]{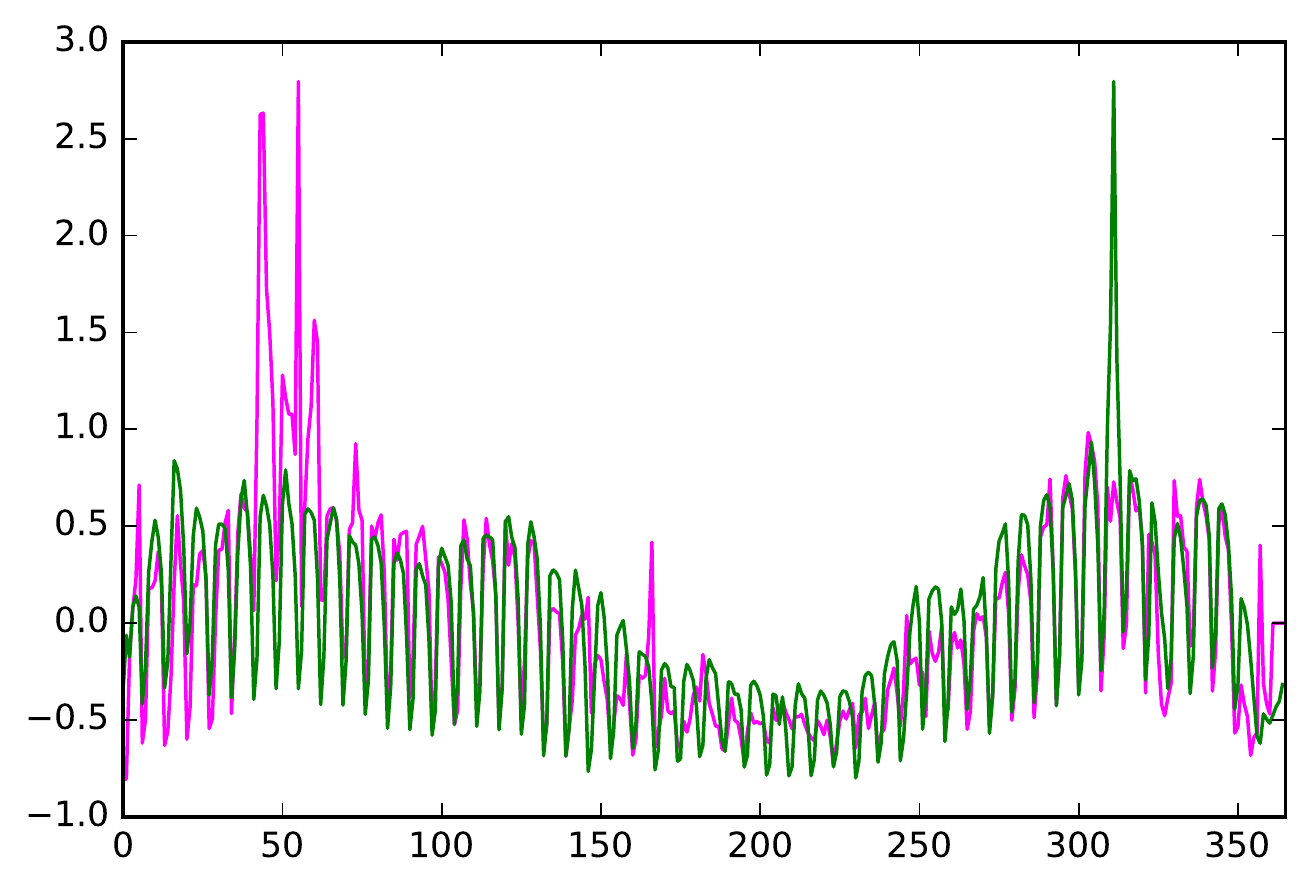}
\vspace{-.5cm}
\caption{Andrew Jackson 2014} 
\label{fig:ex_longrange_c}
\end{subfigure}

\medskip
\vspace{-.2cm}

\begin{subfigure}[t]{0.31\linewidth}
\includegraphics[width=\linewidth, height=3cm]{images/example_preds/example_oos_3.pdf}
\vspace{-.5cm}
\caption{April 2014}
\label{fig:ex_longrange_d}
\end{subfigure}
\hfill
\begin{subfigure}[t]{0.31\textwidth}
\includegraphics[width=\linewidth, height=3cm]{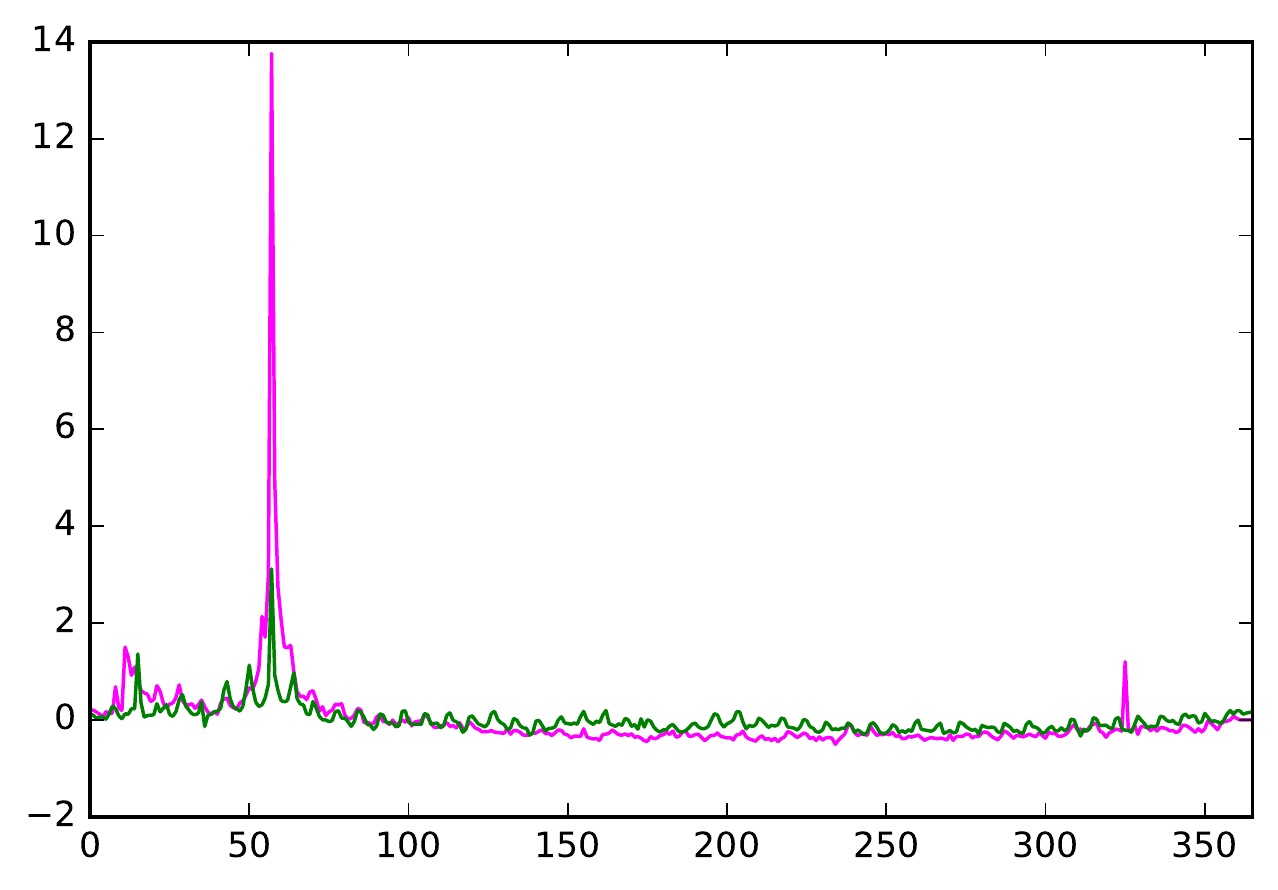}
\vspace{-.5cm}
\caption{Academy Award for Best Picture 2014} 
\label{fig:ex_longrange_e}
\end{subfigure}
\hfill
\begin{subfigure}[t]{0.31\textwidth}
\includegraphics[width=\linewidth, height=3cm]{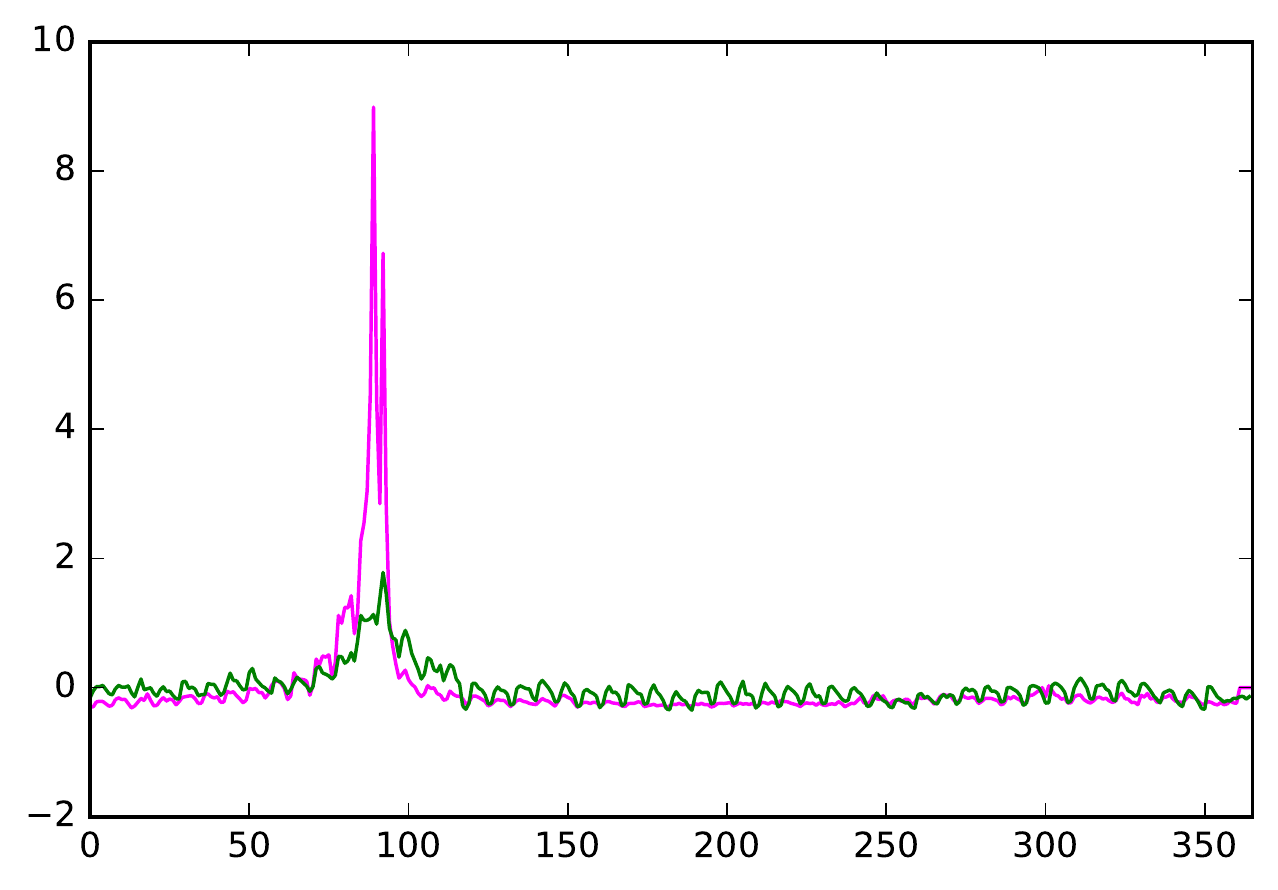}
\vspace{-.5cm}
\caption{Qingming Festival 2014} 
\label{fig:ex_longrange_f}
\end{subfigure}

\medskip
\vspace{-.2cm}
%\begin{figure}[th!]
%\begin{center}

\begin{subfigure}[t]{0.31\linewidth}
\includegraphics[width=\linewidth, height=3cm]{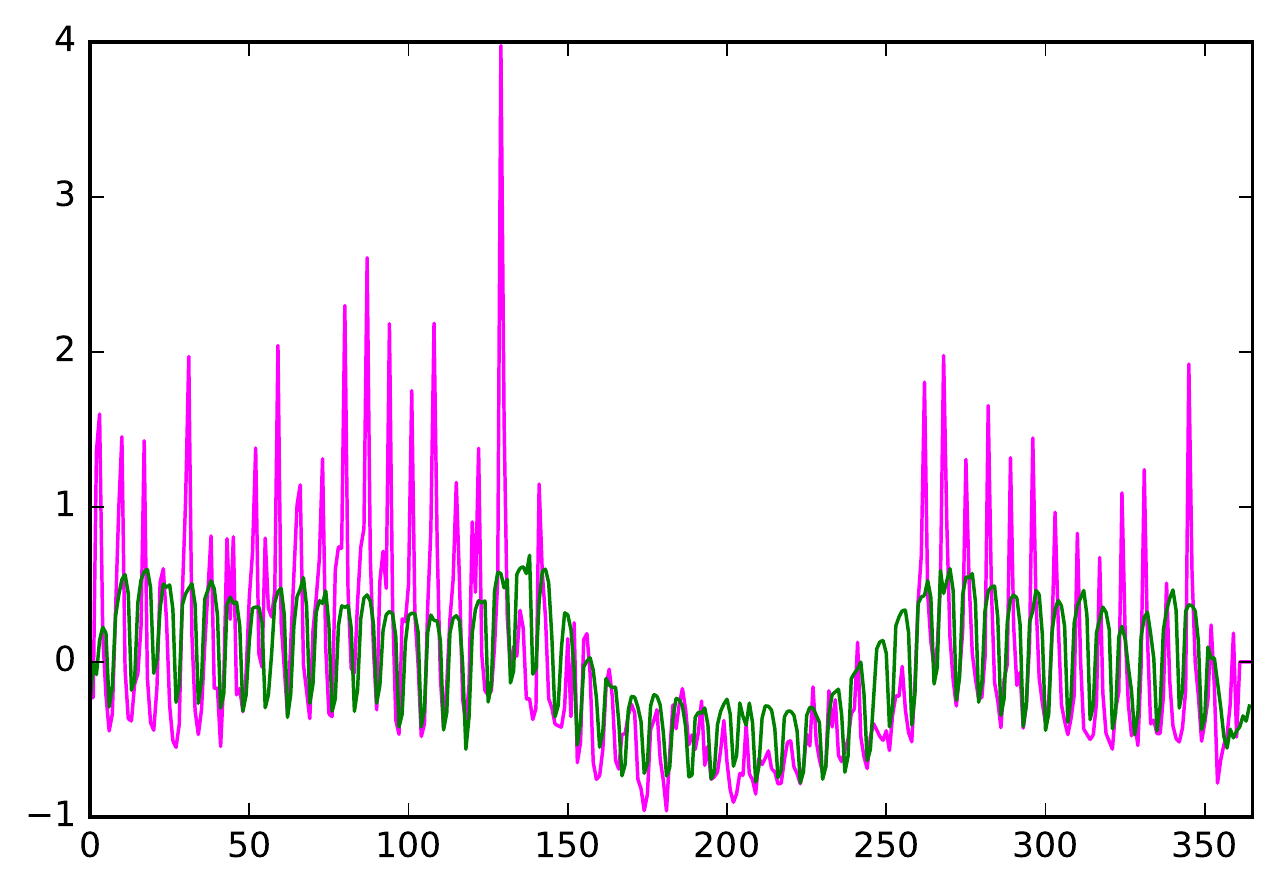}
\vspace{-.5cm}
\caption{NCIS: Los Angeles 2014}
\label{fig:ex_longrange_g}
\end{subfigure}
\hfill
\begin{subfigure}[t]{0.31\textwidth}
\includegraphics[width=\linewidth, height=3cm]{images/example_preds/example_oos_7.pdf}
\vspace{-.5cm}
\caption{Baseball 2014} 
\label{fig:ex_longrange_h}
\end{subfigure}
\hfill
\begin{subfigure}[t]{0.31\textwidth}
\includegraphics[width=\linewidth, height=3cm]{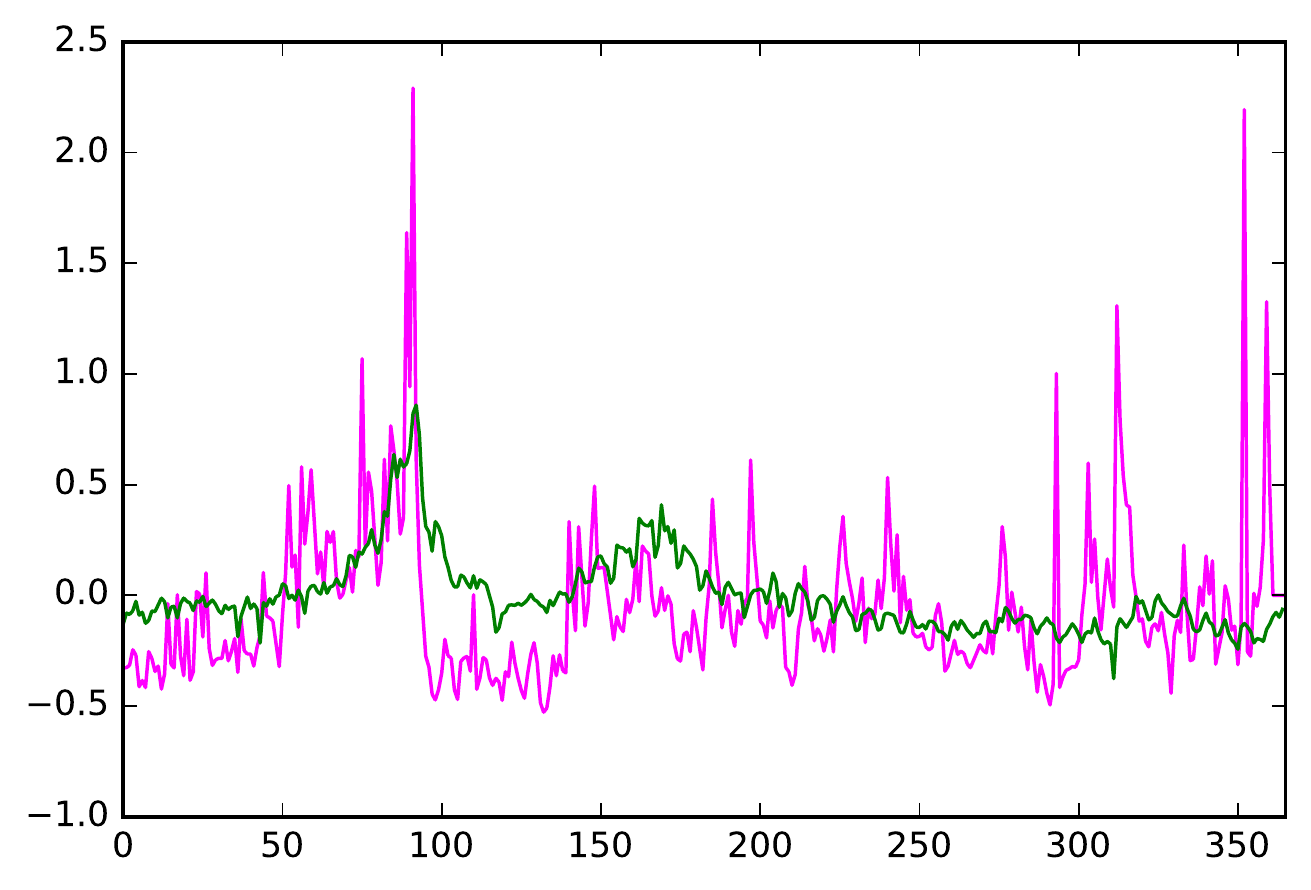}
\vspace{-.5cm}
\caption{Indian national cricket team 2014} 
\label{fig:ex_longrange_i}
\end{subfigure}

\vspace{-.2cm}
\caption{Predictions of the MF + low-rank regression model on Wikipedia page traffic data set for the long-range challenge. The \textcolor{magenta}{observed time series} is in magenta and \textcolor{ForestGreen}{predictions} are overlayed in green. In the top row we observe accurate and relatively similar forecasts for pages corresponding to three US presidents; the large predicted spike in each case most likely corresponds to the date of the US general elections. The middle row contains three examples of series that exhibit a single, strong spike - a relatively common feature in this data. The MF + low-rank model correctly predicts the spike (though not the full extent of its magnitude) in each case; we note that for the Academy Awards page, it even picks out the nomination date in mid-January. In the bottom row, we show three examples of series that have a natural but unique seasonality, either corresponding to a television or sports season. For each series, the MF + low-rank model generates a forecast that reproduces this seasonal structure. }
\label{fig:mflrr_longrange_example_predictions}
\end{center}
\end{figure*}
}

\removed{
\begin{figure*}[t!]
\begin{center}

\begin{subfigure}[t]{0.31\linewidth}
\includegraphics[width=\linewidth, height=3cm]{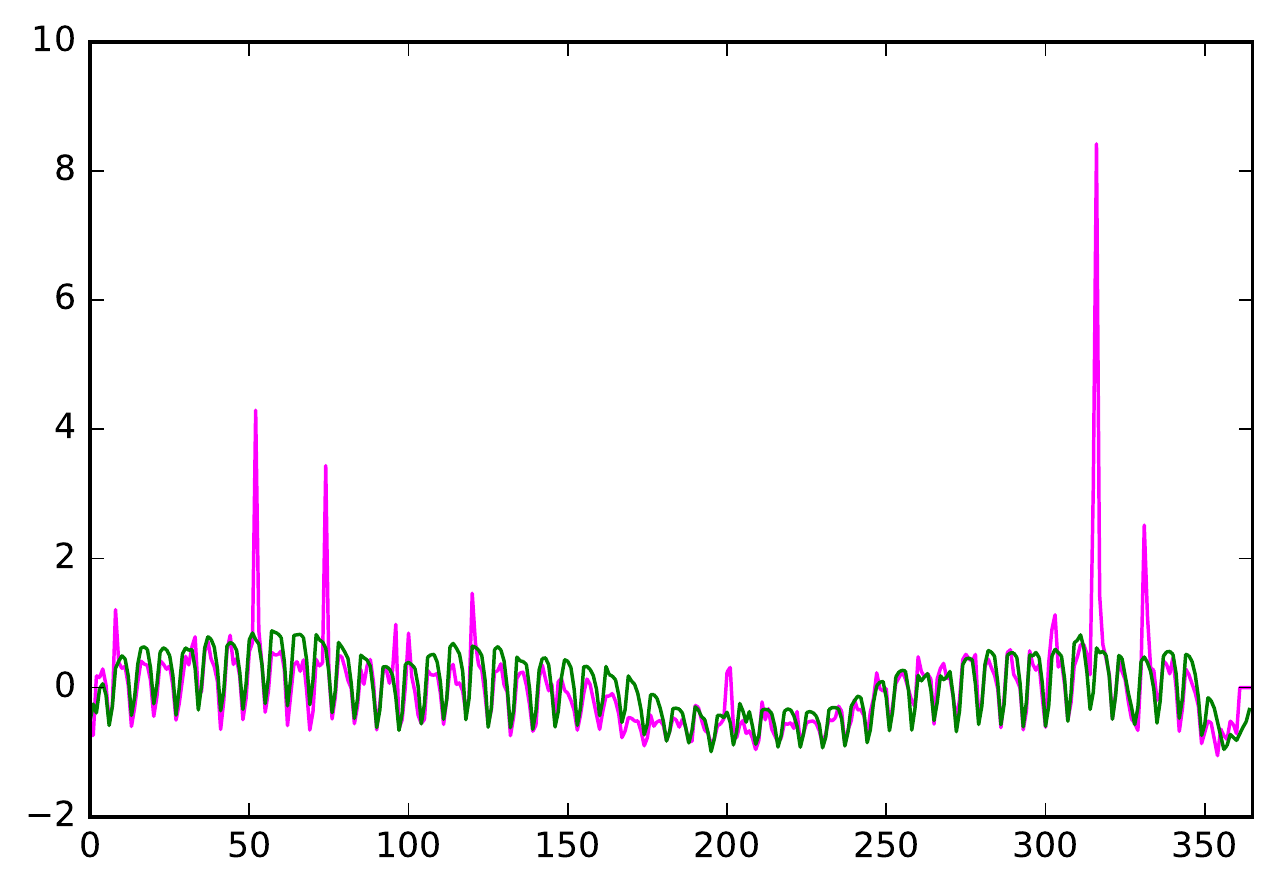}
\vspace{-.5cm}
\caption{Napoleon 2014}
\label{fig:ex_cs_a}
\end{subfigure}
\hfill
\begin{subfigure}[t]{0.31\linewidth}
\includegraphics[width=\linewidth, height=3cm]{images/example_preds/example_cs_1.pdf}
\vspace{-.5cm}
\caption{Miles Davis 2014}
\label{fig:ex_cs_b}
\end{subfigure}
\hfill
\begin{subfigure}[t]{0.31\textwidth}
\includegraphics[width=\linewidth, height=3cm]{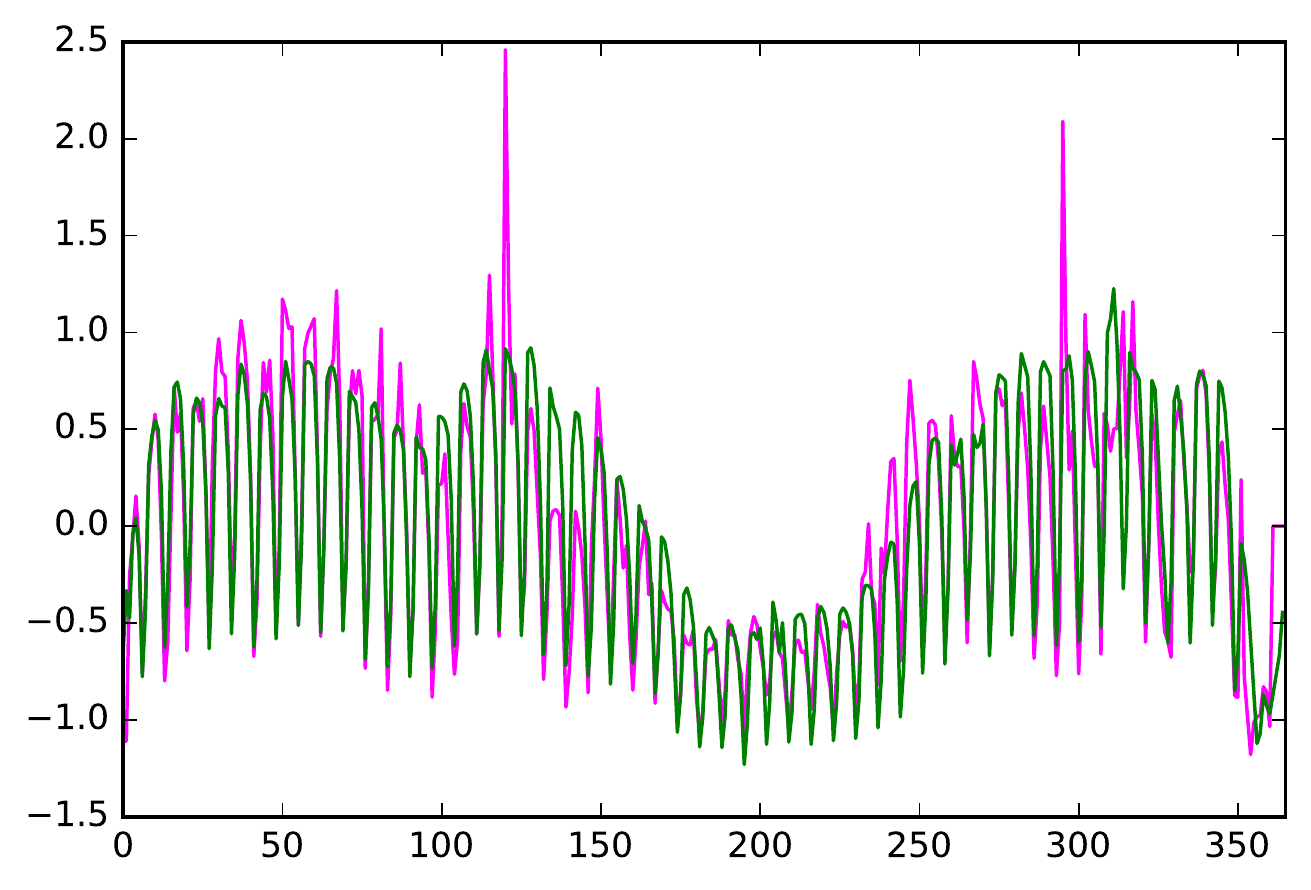}
\vspace{-.5cm}
\caption{Karl Marx 2014} 
\label{fig:ex_cs_c}
\end{subfigure}

\medskip
\vspace{-.2cm}

\begin{subfigure}[t]{0.31\linewidth}
\includegraphics[width=\linewidth, height=3cm]{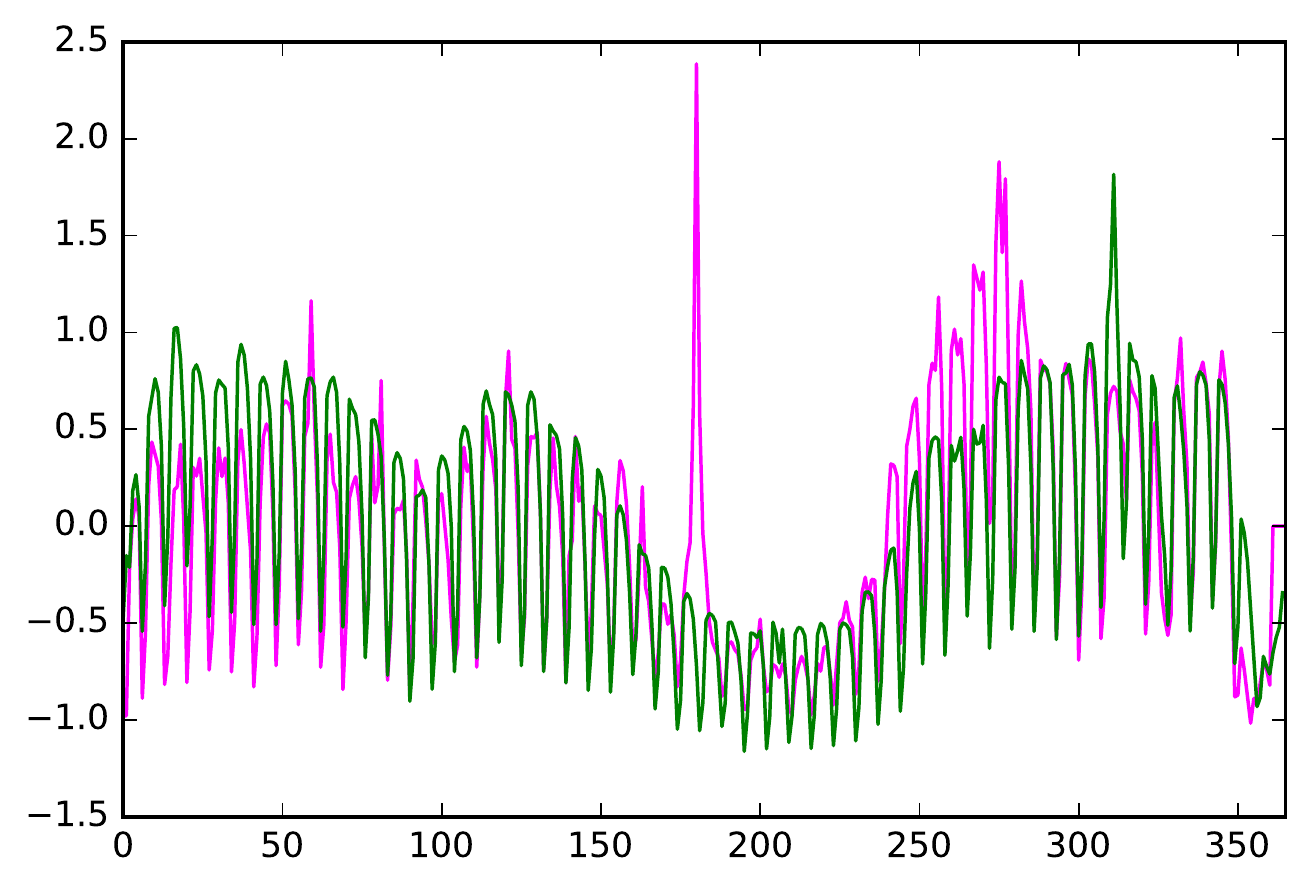}
\vspace{-.5cm}
\caption{American Revolution 2014}
\label{fig:ex_cs_d}
\end{subfigure}
\hfill
\begin{subfigure}[t]{0.31\textwidth}
\includegraphics[width=\linewidth, height=3cm]{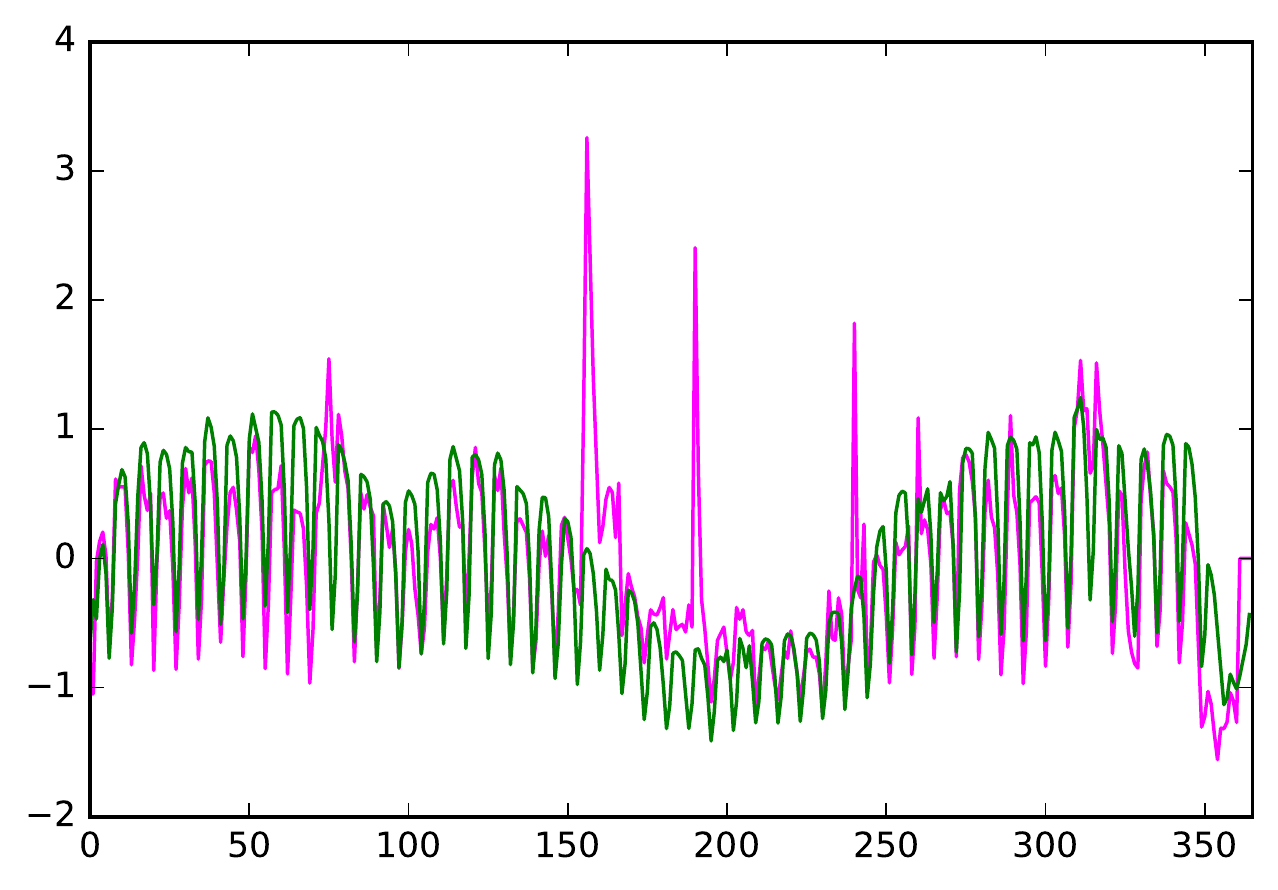}
\vspace{-.5cm}
\caption{French Revolution 2014} 
\label{fig:ex_cs_e}
\end{subfigure}
\hfill
\begin{subfigure}[t]{0.31\textwidth}
\includegraphics[width=\linewidth, height=3cm]{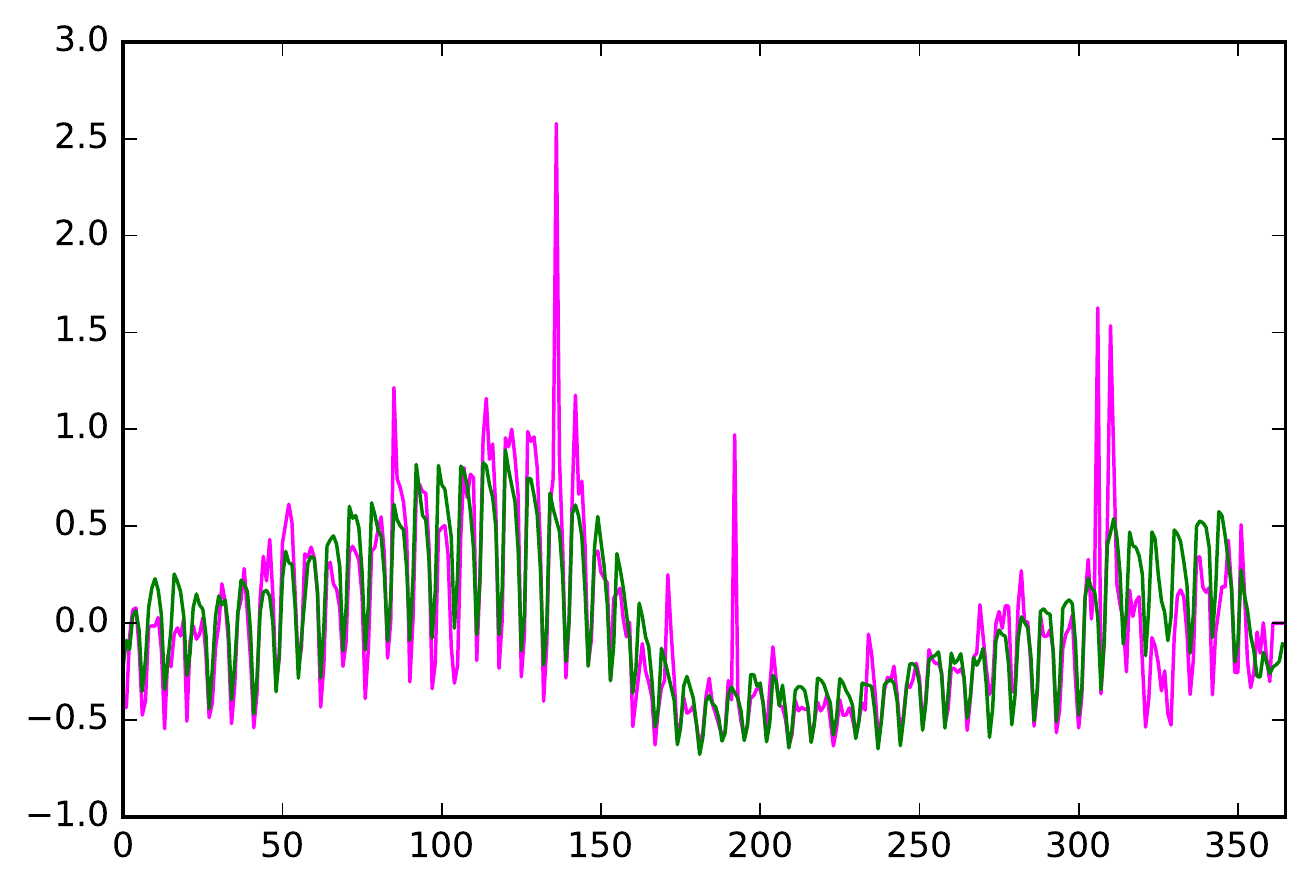}
\vspace{-.5cm}
\caption{Korean War 2014} 
\label{fig:ex_cs_f}
\end{subfigure}

\medskip
\vspace{-.2cm}
%\begin{figure}[th!]
%\begin{center}

\begin{subfigure}[t]{0.31\linewidth}
\includegraphics[width=\linewidth, height=3cm]{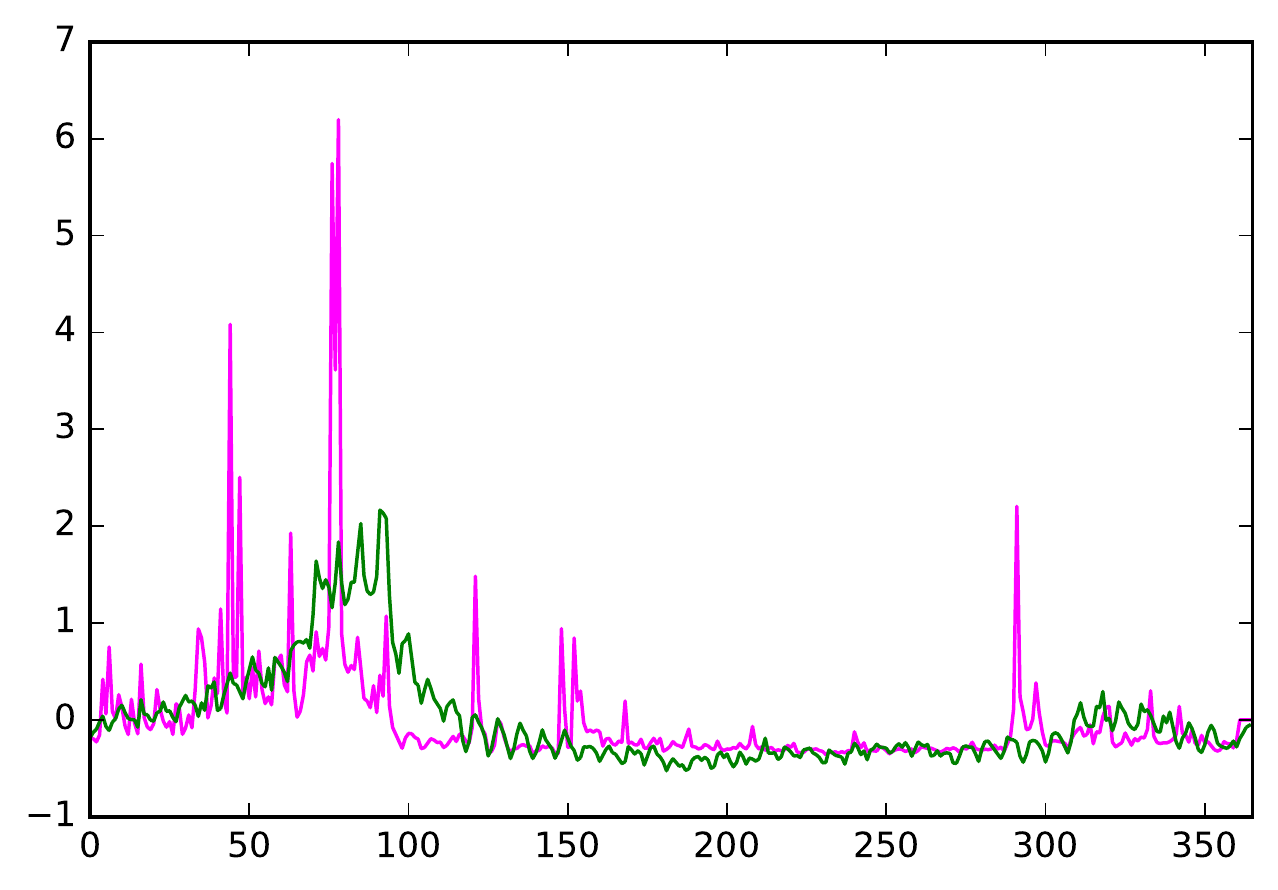}
\vspace{-.5cm}
\caption{Roy Williams (coach) 2014}
\label{fig:ex_cs_g}
\end{subfigure}
\hfill
\begin{subfigure}[t]{0.31\textwidth}
\includegraphics[width=\linewidth, height=3cm]{images/example_preds/example_cs_7.pdf}
\vspace{-.5cm}
\caption{WrestleMania 2014} 
\label{fig:ex_cs_h}
\end{subfigure}
\hfill
\begin{subfigure}[t]{0.31\textwidth}
\includegraphics[width=\linewidth, height=3cm]{images/example_preds/example_cs_8.pdf}
\vspace{-.5cm}
\caption{Johan Cruyff 2014} 
\label{fig:ex_cs_i}
\end{subfigure}

\vspace{-.2cm}
\caption{Predictions of the MF + low-rank regression model on Wikipedia page traffic data set for the cold-start challenge. The \textcolor{magenta}{observed time series} is in magenta and \textcolor{ForestGreen}{predictions} are overlayed in green. In the top row, we observe the MF + low-rank model producing similar and accurate seasonal profile forecasts for three previously unobserved pages corresponding to historical figures. In the middle row, we see two similar forecasts for the American and French Revolutions, likely corresponding to their similarity in metadata space, while the model comes up with a notably different but highly accurate profile for the Korean War. In the bottom row, the MF + low-rank model correctly predicts the location of a temporally distant spike despite not having previously observed any of the series; in this case, each corresponds to a popular sporting event related to the page (US college basketball for Roy Williams, wrestling for WrestleMania, and the World Cup for Johan Cruyff).}
\label{fig:mflrr_coldstart_example_predictions}
\end{center}
\end{figure*}

\begin{figure*}[t!]
\begin{center}

\begin{subfigure}[t]{0.31\linewidth}
\includegraphics[width=\linewidth, height=3.5cm]{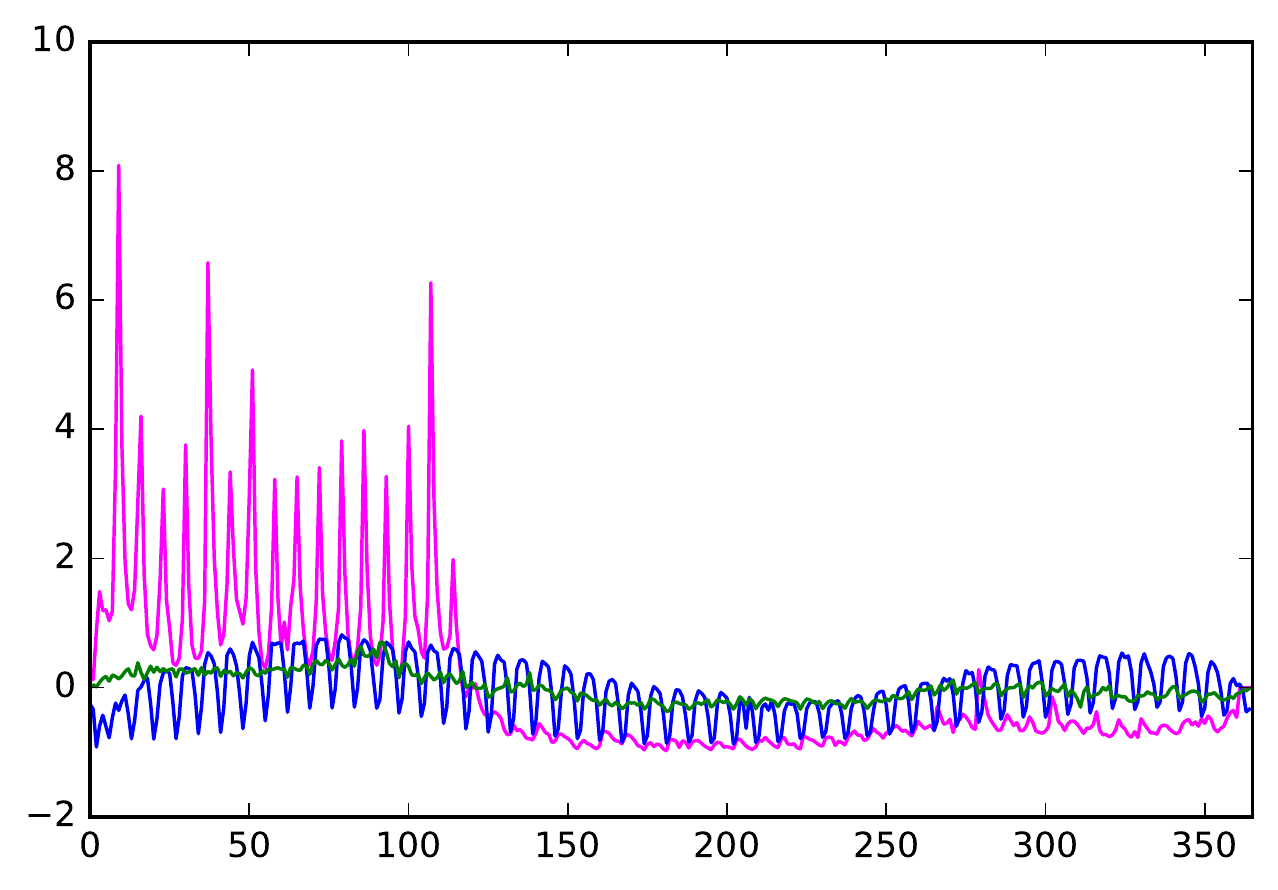}
\vspace{-.5cm}
\caption{List of Archer Episodes 2014}
\label{fig:best_trmf_a}
\end{subfigure}
\hfill
\begin{subfigure}[t]{0.31\textwidth}
\includegraphics[width=\linewidth, height=3.5cm]{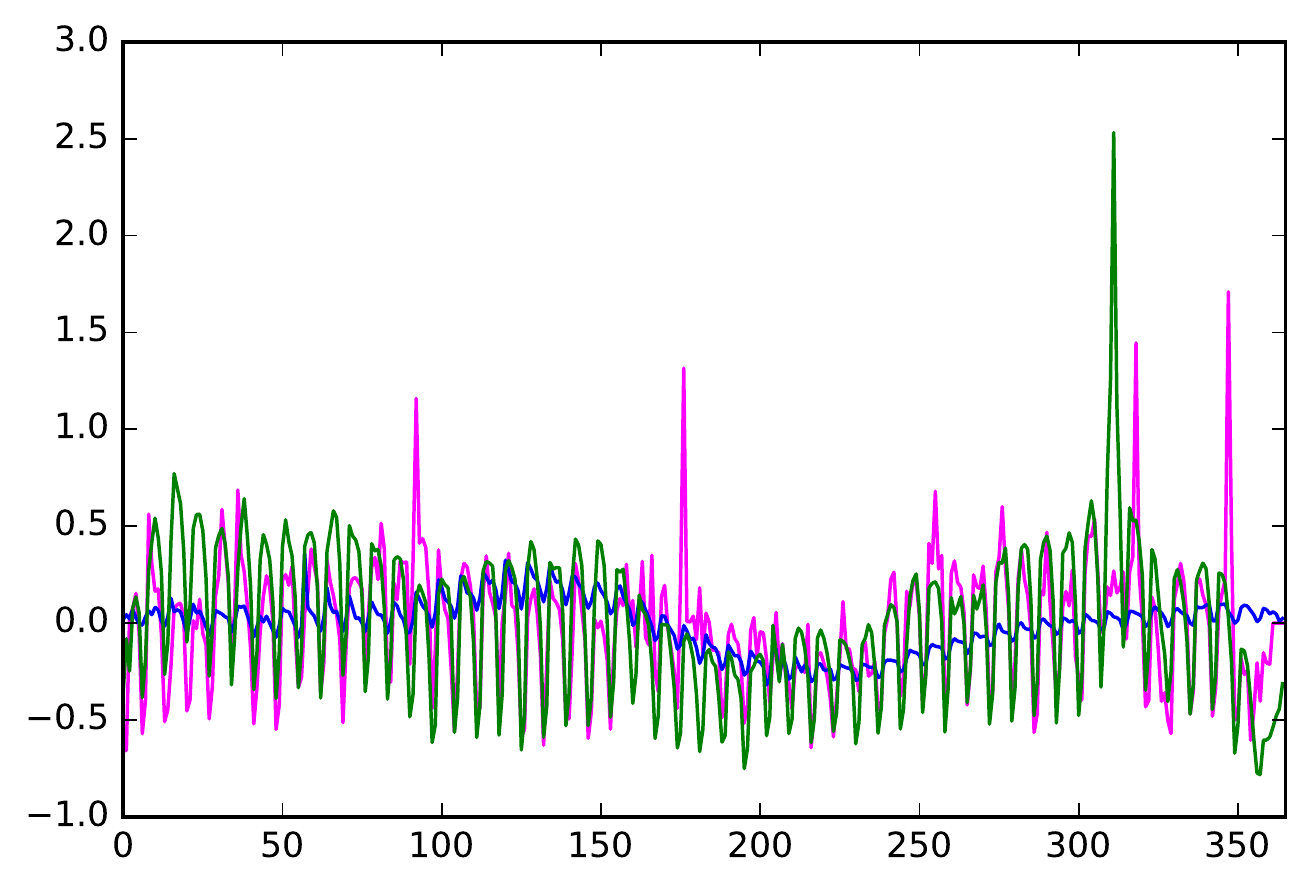}
\vspace{-.5cm}
\caption{Puerto Rico 2014} 
\label{fig:best_trmf_b}
\end{subfigure}
\hfill
\begin{subfigure}[t]{0.31\textwidth}
\includegraphics[width=\linewidth, height=3.5cm]{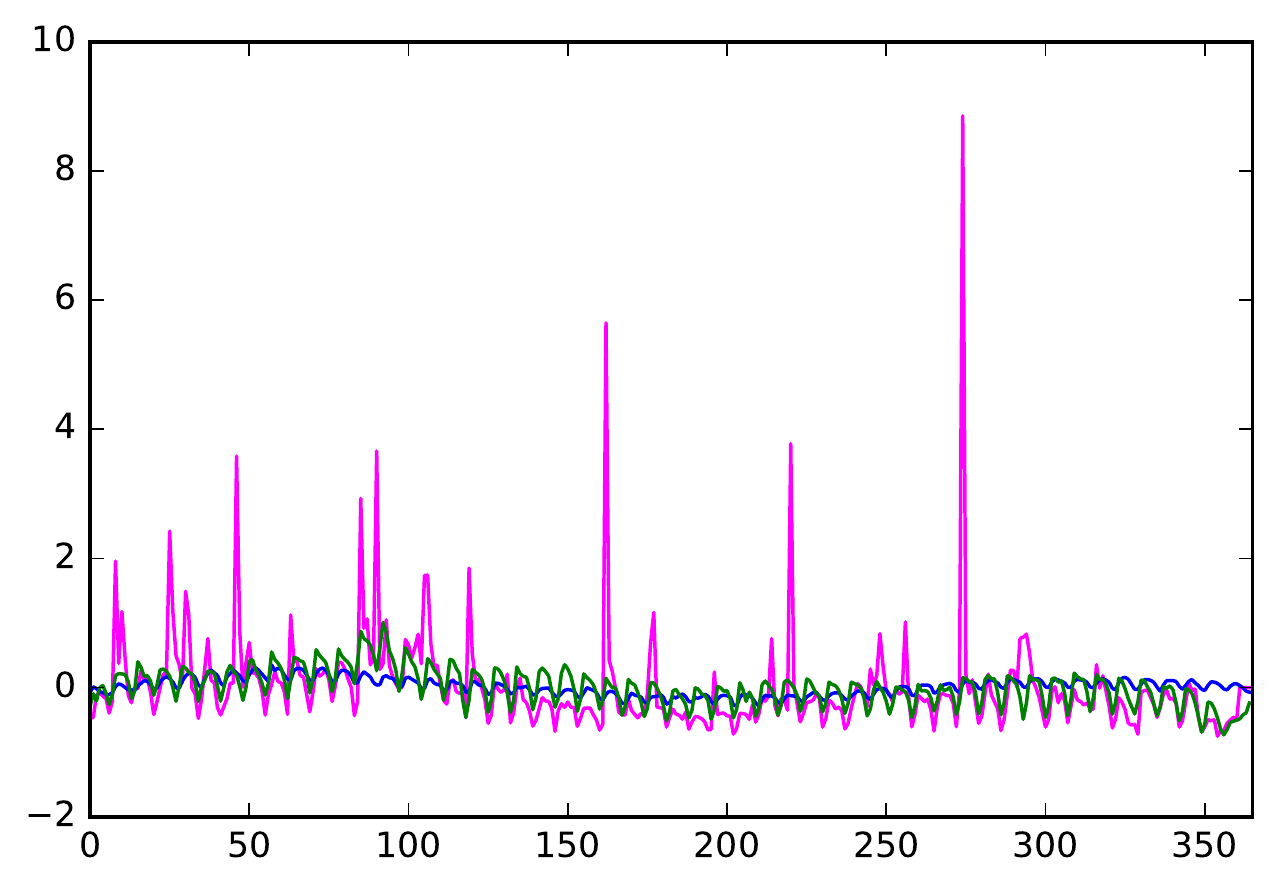}
\vspace{-.5cm}
\caption{Easter Island 2014} 
\label{fig:best_trmf_c}
\end{subfigure}

\medskip
\vspace{-.2cm}
%\begin{figure}[th!]
%\begin{center}

\begin{subfigure}[t]{0.31\linewidth}
\includegraphics[width=\linewidth, height=3.5cm]{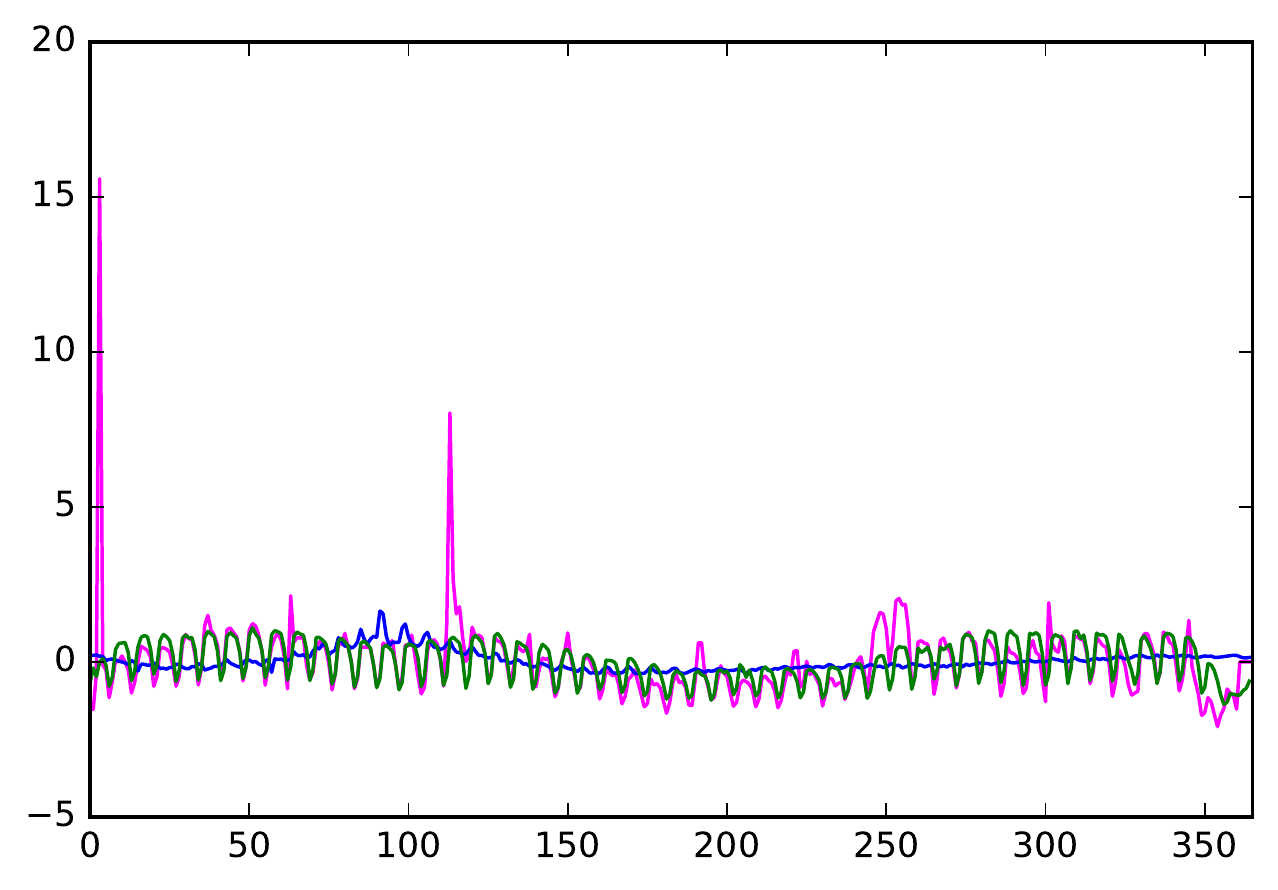}
\vspace{-.5cm}
\caption{Dopamine 2014}
\label{fig:best_trmf_d}
\end{subfigure}
\qquad
\begin{subfigure}[t]{0.31\textwidth}
\includegraphics[width=\linewidth, height=3.5cm]{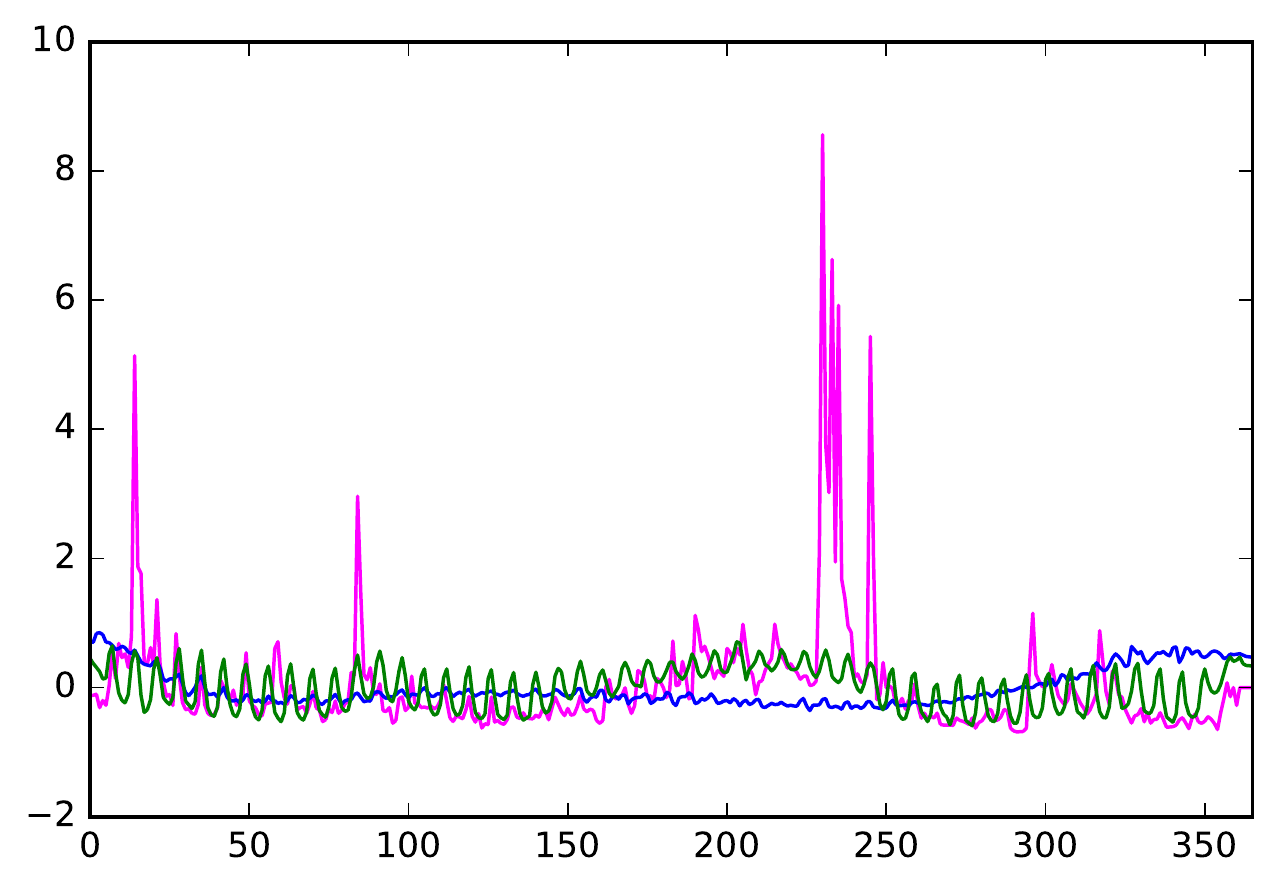}
\vspace{-.5cm}
\caption{Nathan Kress 2014} 
\label{fig:best_trmf_e}
\end{subfigure}

\vspace{-.2cm}
\caption{Predictions of the TRMF and MF + low-rank regression model on Wikipedia page traffic data set for the long-range challenge. The \textcolor{magenta}{observed time series} is in magenta, while TRMF \textcolor{blue}{predictions} are in blue and MF + low-rank \textcolor{ForestGreen}{predictions} are overlayed in green. The series plotted in this figure correspond to the five series mdAPE errors closest to the $10^{th}$ quantile of mdAPE errors over all test series for TRMF, thus they represent a collection of some of the ``best" predictions for this method. However, when we simultaneously plot MF + low-rank predictions, we observe that our approach consistently generates forecasts that more faithfully reproduce the true seasonal and oscillatory profiles of the test series. These results underscore the importance of using long-range techniques over even sophisticated step-ahead forecasters for the challenge of long-range time series prediction.}
\label{fig:best_trmf_predictions}
\end{center}
\end{figure*}

\begin{figure*}[t!]
\begin{center}

\begin{subfigure}[t]{0.31\linewidth}
\includegraphics[width=\linewidth, height=3cm]{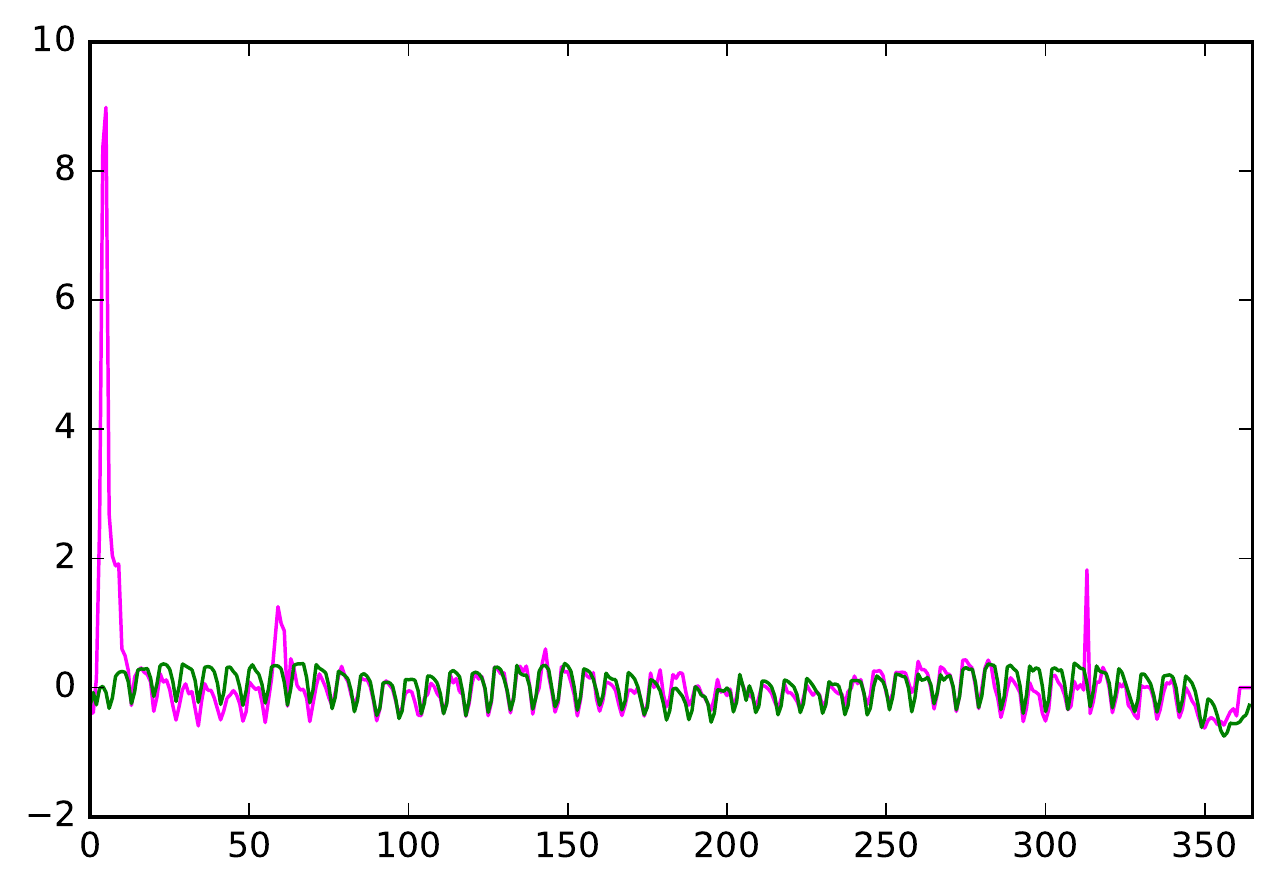}
\vspace{-.5cm}
\caption{Niagara Falls 2014}
\label{fig:mflrr_qtls_a}
\end{subfigure}
\hfill
\begin{subfigure}[t]{0.31\linewidth}
\includegraphics[width=\linewidth, height=3cm]{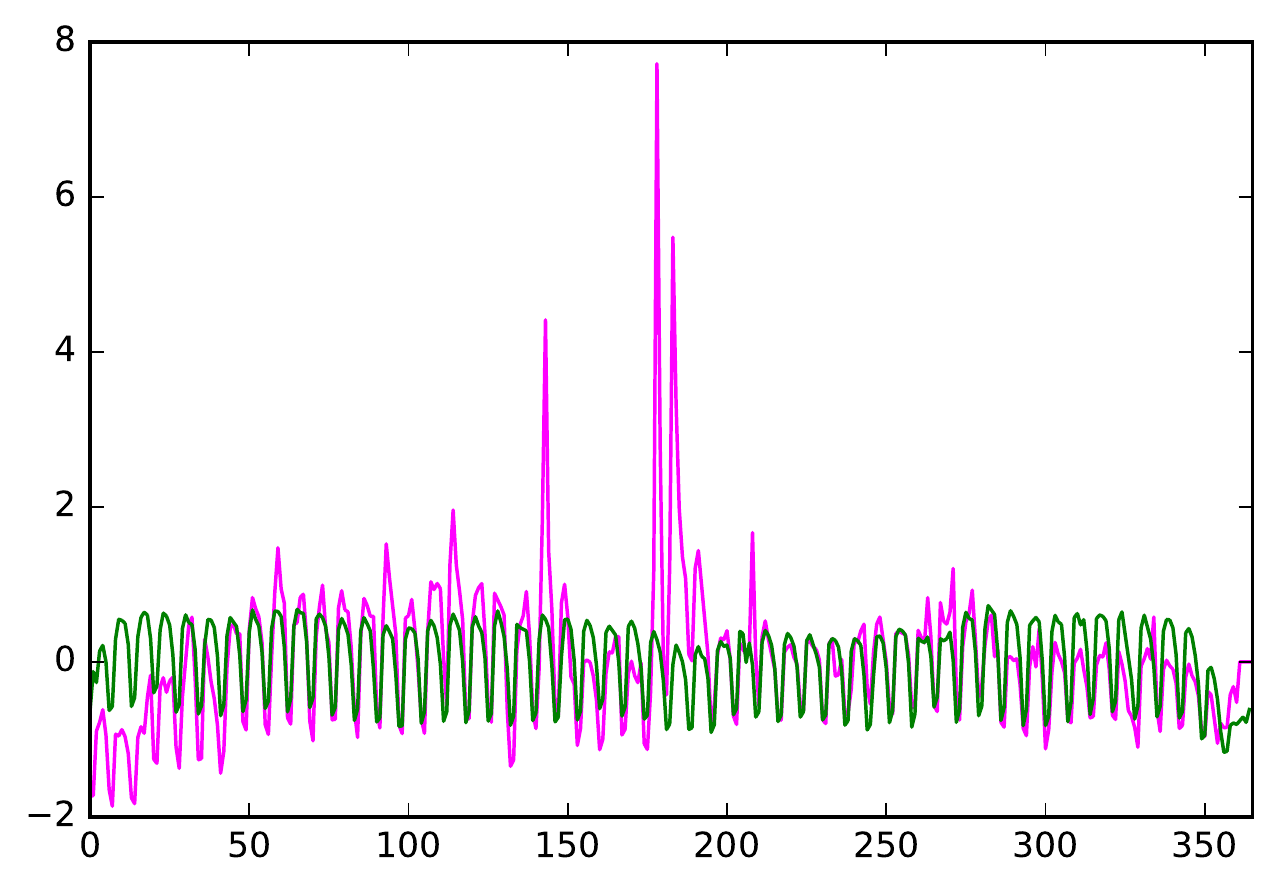}
\vspace{-.5cm}
\caption{Scabies 2014}
\label{fig:mflrr_qtls_b}
\end{subfigure}
\hfill
\begin{subfigure}[t]{0.31\textwidth}
\includegraphics[width=\linewidth, height=3cm]{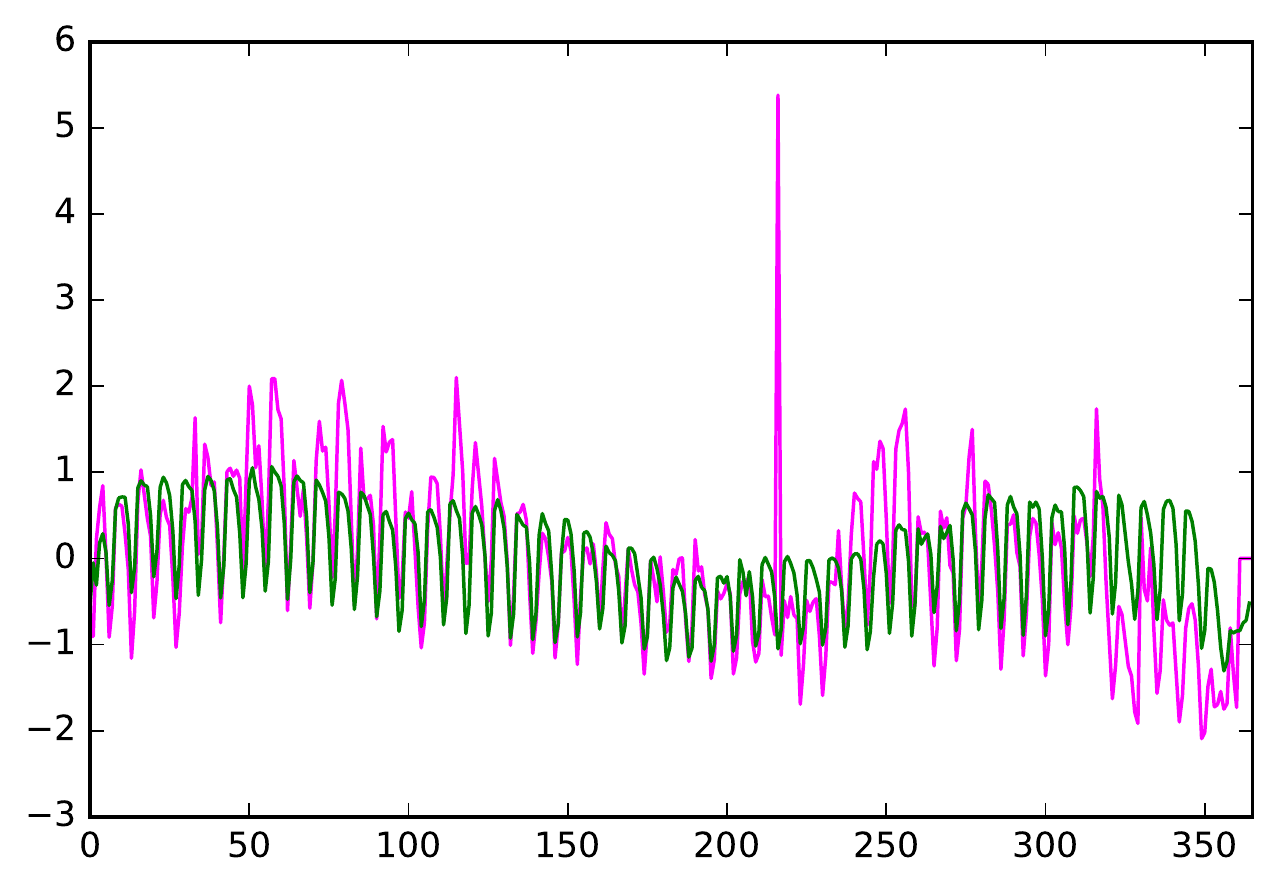}
\vspace{-.5cm}
\caption{List of countries by GDP (nominal) per capita 2014} 
\label{fig:mflrr_qtls_c}
\end{subfigure}

\medskip
\vspace{-.2cm}

\begin{subfigure}[t]{0.31\linewidth}
\includegraphics[width=\linewidth, height=3cm]{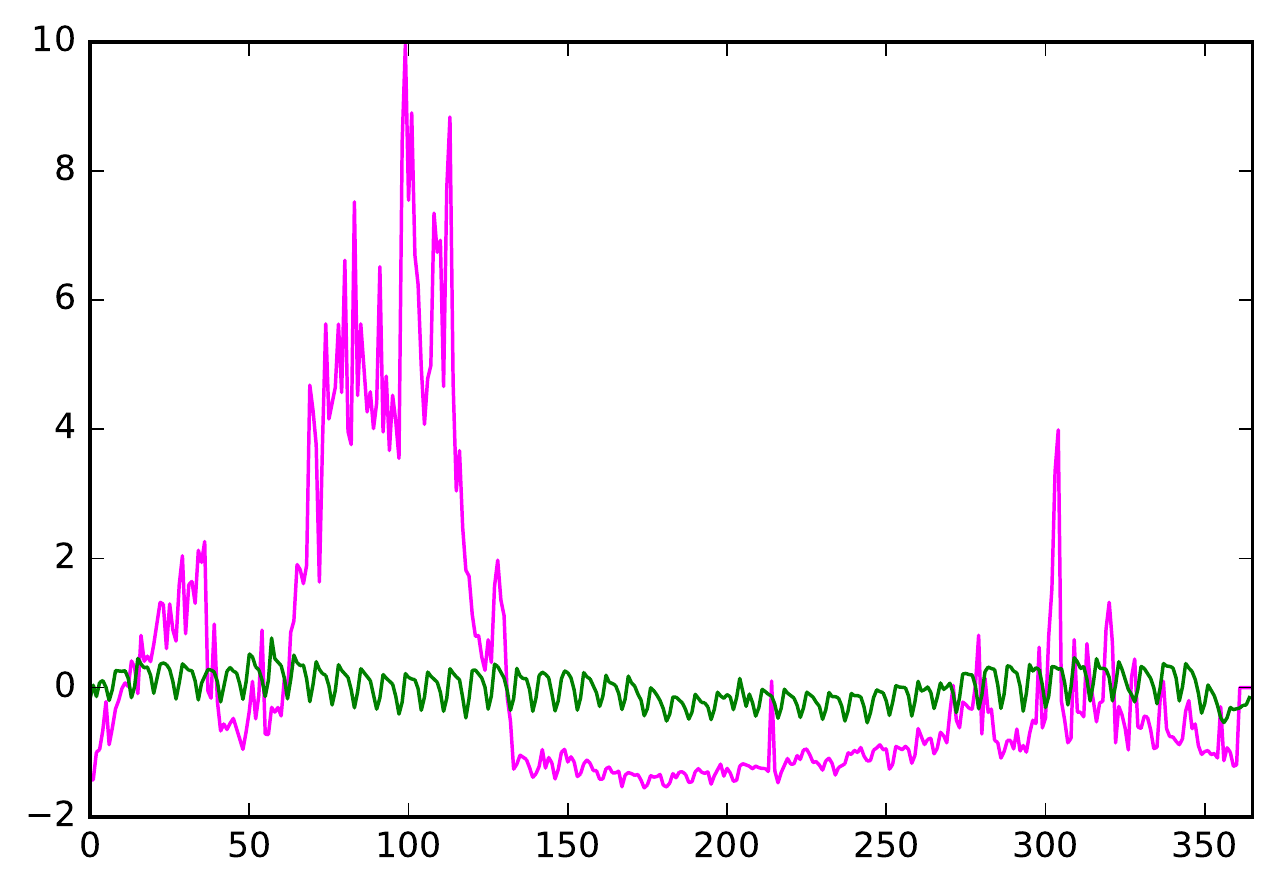}
\vspace{-.5cm}
\caption{Film 2014}
\label{fig:mflrr_qtls_d}
\end{subfigure}
\hfill
\begin{subfigure}[t]{0.31\textwidth}
\includegraphics[width=\linewidth, height=3cm]{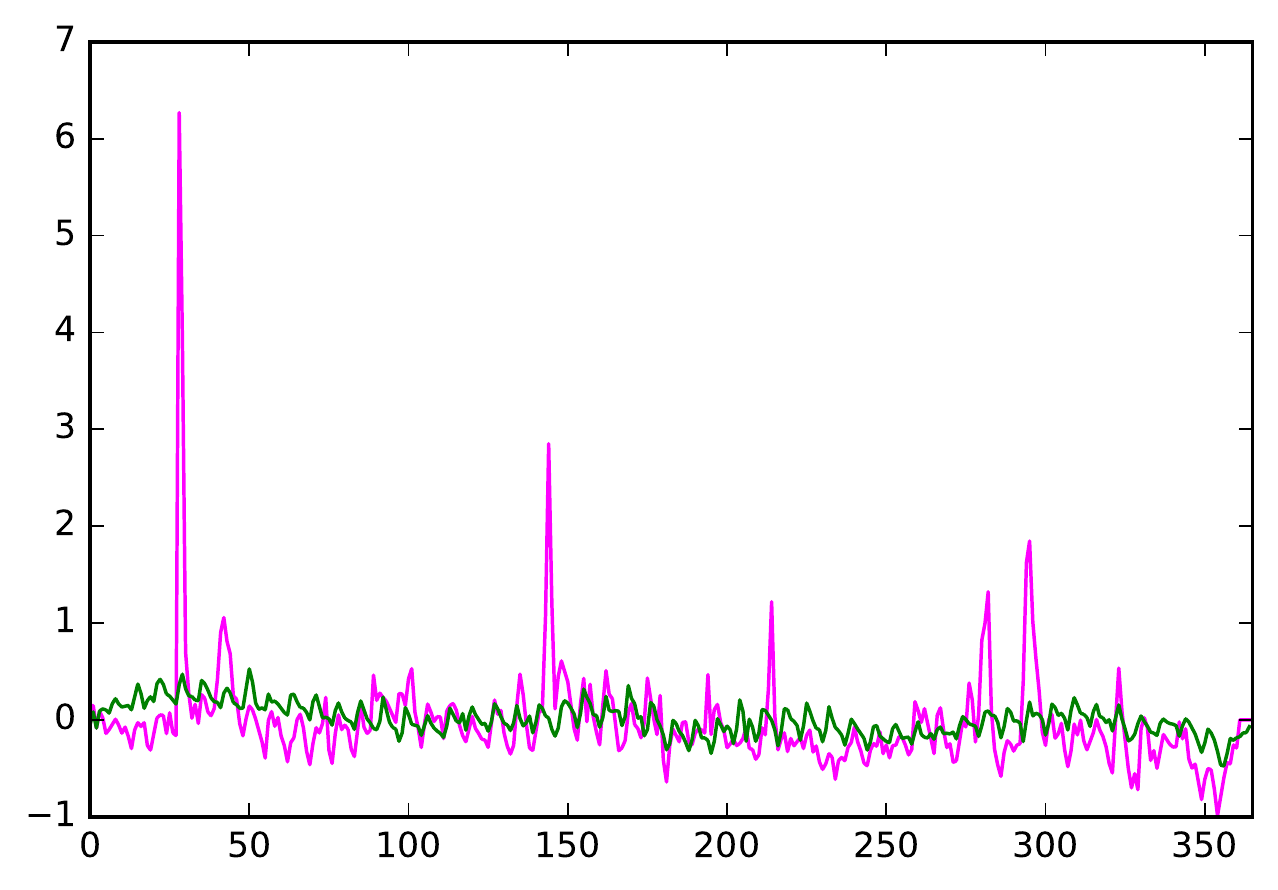}
\vspace{-.5cm}
\caption{Asexuality 2014} 
\label{fig:mflrr_qtls_e}
\end{subfigure}
\hfill
\begin{subfigure}[t]{0.31\textwidth}
\includegraphics[width=\linewidth, height=3cm]{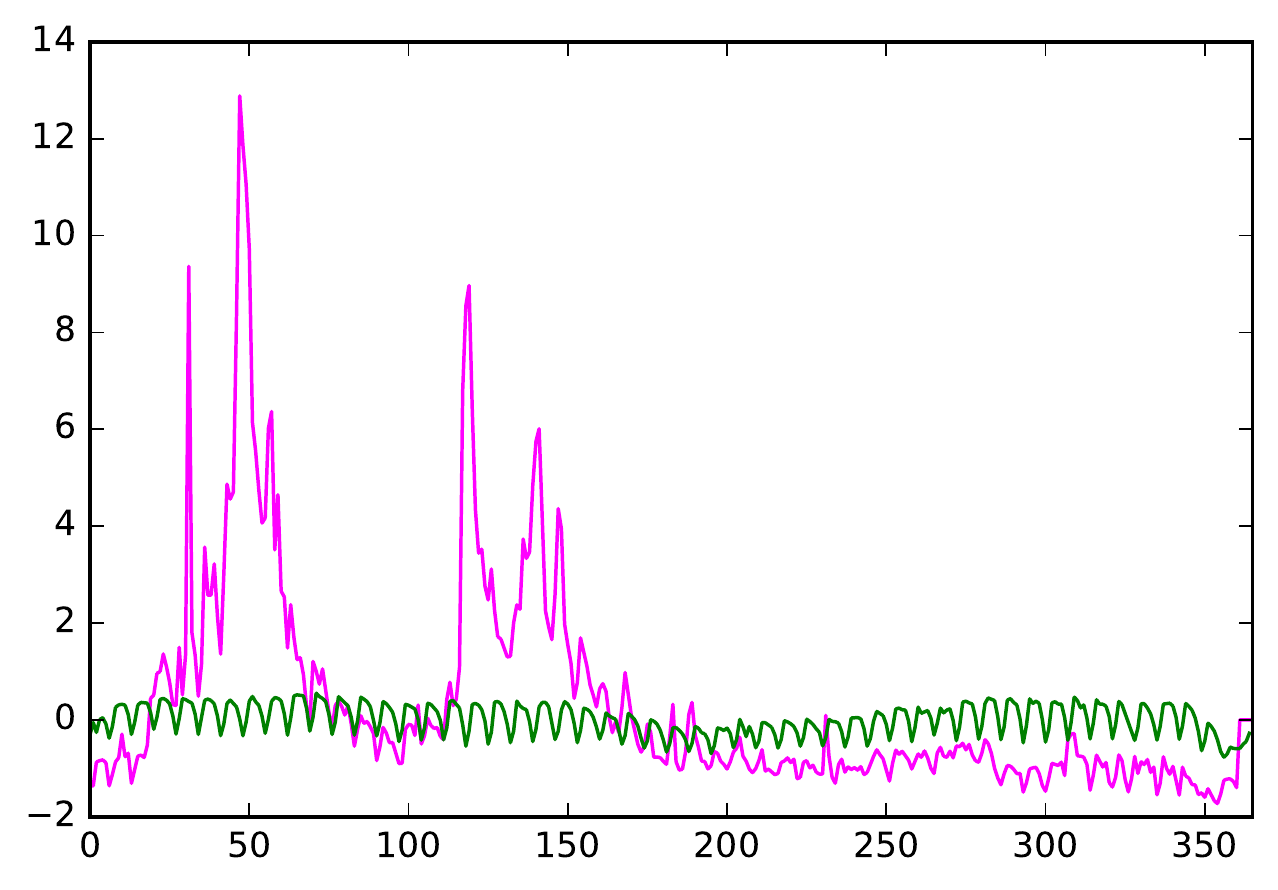}
\vspace{-.5cm}
\caption{Pompeii 2014} 
\label{fig:mflrr_qtls_f}
\end{subfigure}

\medskip
\vspace{-.2cm}
%\begin{figure}[th!]
%\begin{center}

\begin{subfigure}[t]{0.31\linewidth}
\includegraphics[width=\linewidth, height=3cm]{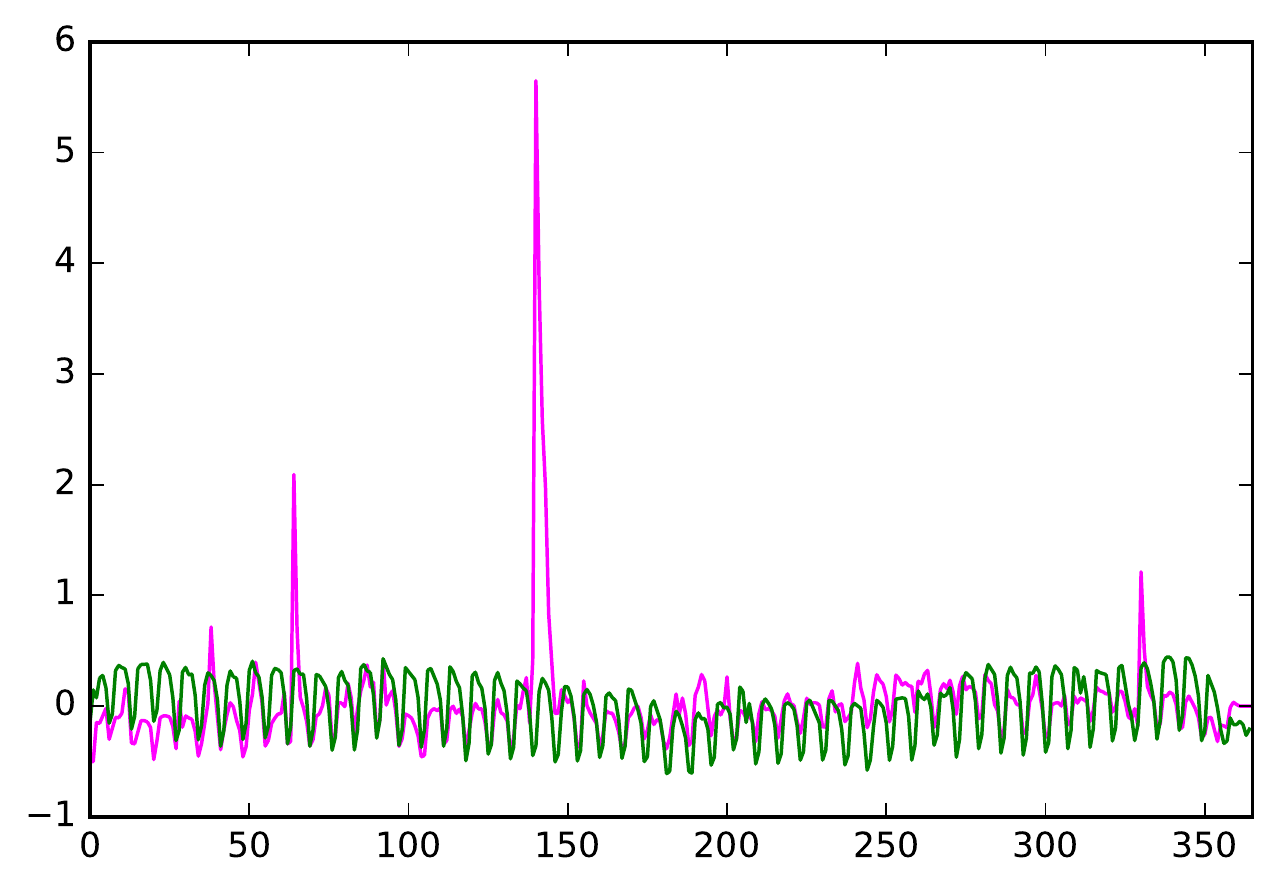}
\vspace{-.5cm}
\caption{Asperger syndrome 2014}
\label{fig:mflrr_qtls_g}
\end{subfigure}
\hfill
\begin{subfigure}[t]{0.31\textwidth}
\includegraphics[width=\linewidth, height=3cm]{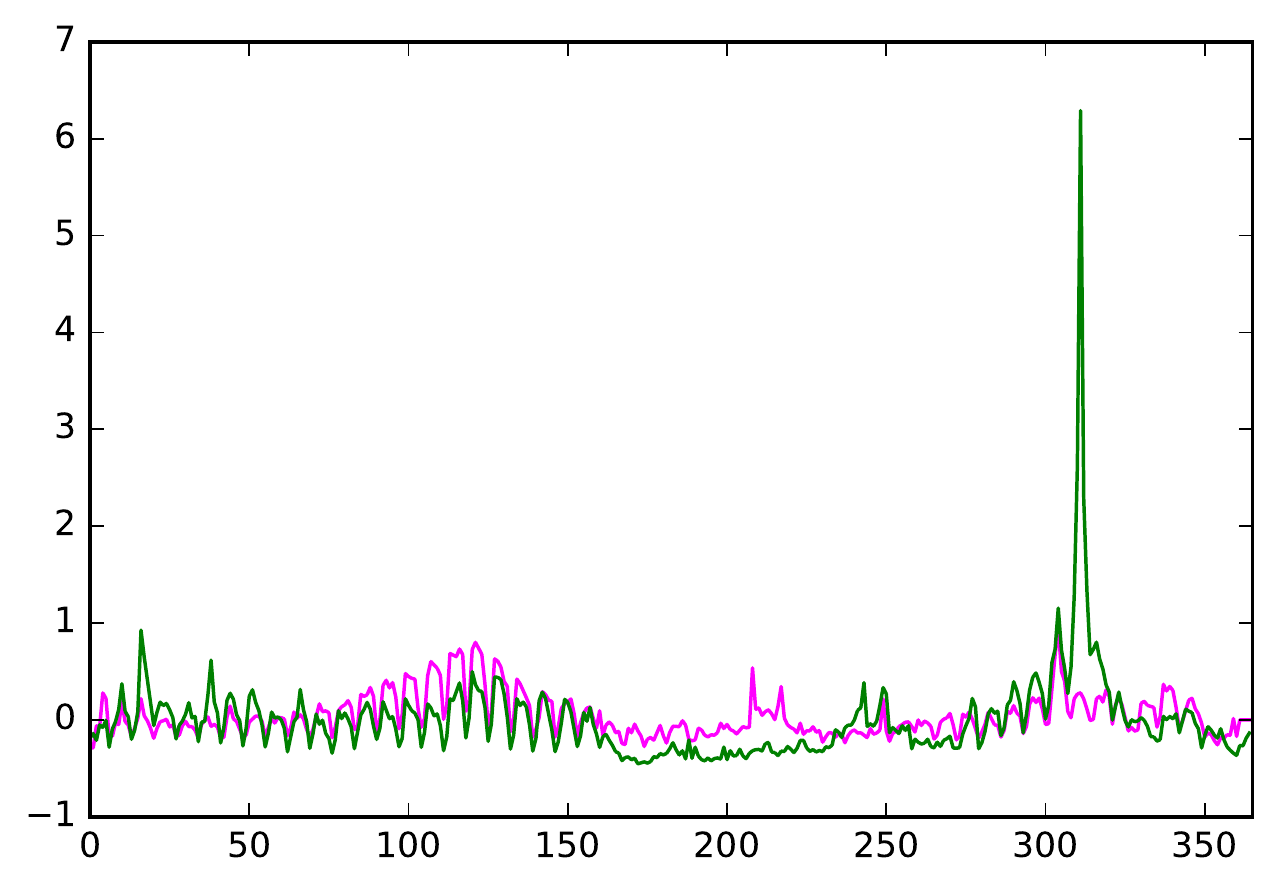}
\vspace{-.5cm}
\caption{United States presidential election 1968 2014} 
\label{fig:mflrr_qtls_h}
\end{subfigure}
\hfill
\begin{subfigure}[t]{0.31\textwidth}
\includegraphics[width=\linewidth, height=3cm]{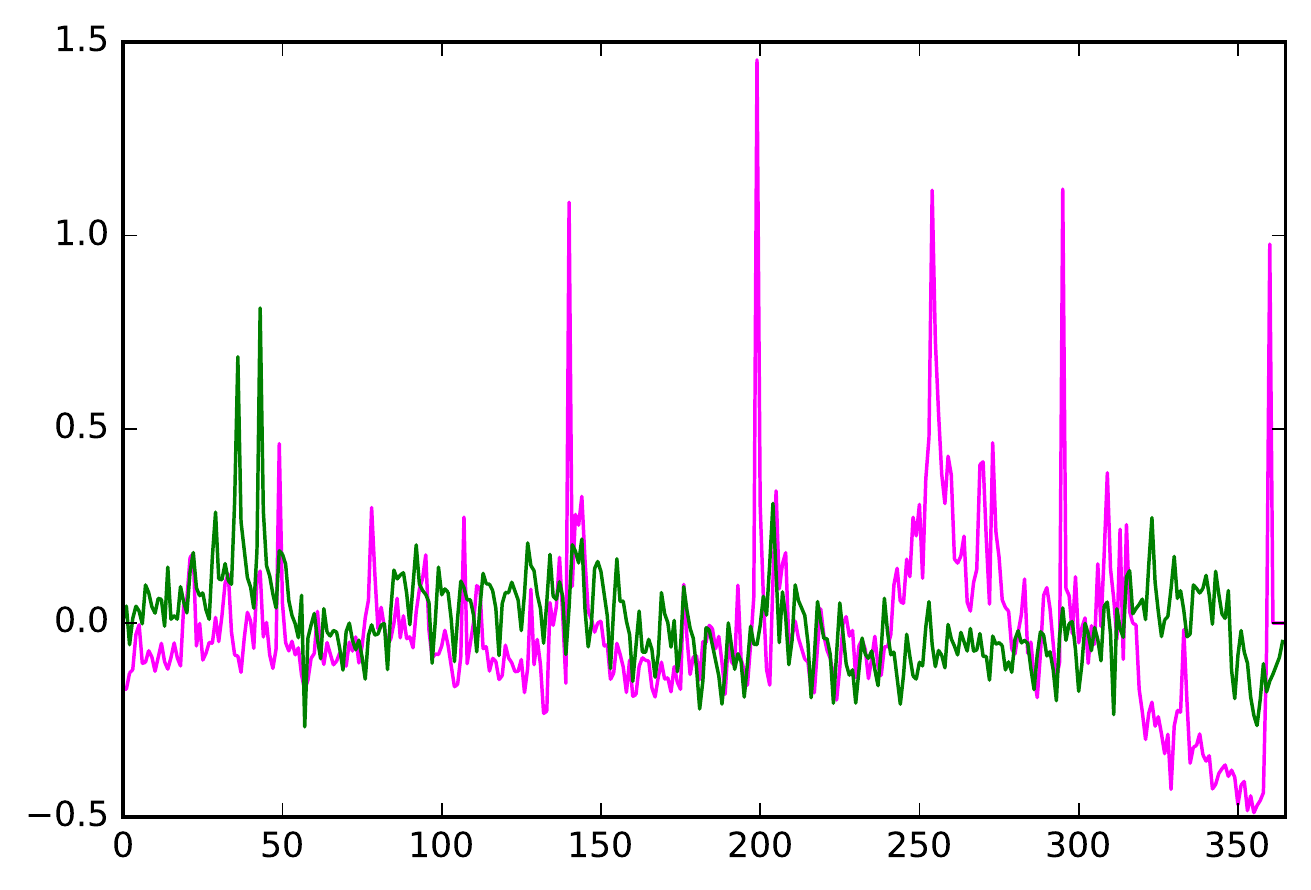}
\vspace{-.5cm}
\caption{Slash (musician) 2014} 
\label{fig:mflrr_qtls_i}
\end{subfigure}

\vspace{-.2cm}
\caption{Predictions of the MF + low-rank regression model on Wikipedia page traffic data set for the long-range challenge. The \textcolor{magenta}{observed time series} is in magenta and \textcolor{ForestGreen}{predictions} are overlayed in green. We plot the three test series closest in to the $10^{th}$ (top row), $50^{th}$ (middle row), and $90^{th}$ (bottom row) quantiles for mdAPE error over all test series for the MF + low-rank model in order to give a visual sense of the distribution of predictive performances on a challenging, real-world data set. }
\label{fig:mflrr_quantile_examples}
\end{center}
\end{figure*}
}
