# Supplementary material for: A Unified Framework for Long Range and Cold Start Forecasting of Seasonal Profiles in Time Series
Source: arXiv:1710.08473 source file (2018-08-26)
Supplement: Supplementary file 2 [file meth_supp.tex]

\removed{
\section{Details on Functional Regression}
\label{appendix:functional_regression}
To enforce smoothness of the regression weights $W_j$ across time steps $j$ we utilize a basis expansion. In particular, we assume that each element of $W_j$ may be written as a linear combination of \emph{basis functions} evaluated at time step $j$. Specifically, we have that element $k$ of vector $W_j$, $W_{jk}$, is written as
 \begin{align}
     W_{jk} = \sum_{h=1}^K b_{h}(j) Q_{hk},
 \end{align}
 where $b_h(j)$ is the $h$th smooth basis function evaluated at time point $j$ and the $Q_{hk}$ are linear combination coefficients that are constant across time. The goal is to learn the basis weights $Q_{hk}$ $\forall h,k$ which fully describes the functional regression model. Under this parameterization, Eq. (3) in the main paper becomes
\begin{align}
Y_{ji} &= \sum_{k=1}^m \sum_{h=1}^K b_h(j) Q_{hk} \phi_{ki} + \veps_{ji}\\
&= B_j^\T Q \phi_i + \veps_{ji},
 \end{align}
where the basis function weights are collected into the matrix $Q$ and here $B_j$ is the vector with elements $B_j = \left(b_{1}(j) ,\ldots, b_{K}(j)\right)$. 
}

\removed{
\section{Framework Optimization Objectives}
Here we provide the specific optimization objectives for all methods shown in Table 1 in the main paper. 
\begin{itemize}
    \item Regression:  
\begin{align*}
\argmin_{W}&\ \frac{1}{2N} \sum_{(j,i) \in \Omega} \left(Y_{ji} - W_j^\T \phi_i \right)^2 + \frac{\lambda_1}{2N}  \|W\|_F^2 
\end{align*}
    \item Matrix factorization + regression:
\begin{align*}
\argmin_{L,R,W}&\ \frac{1}{2N} \sum_{(j,i) \in \Omega} \left(Y_{ji} - L_j^\T R_i - W_j^\T \phi_i \right)^2 + \frac{\lambda_1}{2N}  \|W\|_F^2 + \frac{\lambda_2}{2N}  \left(\|L\|_F^2 + \|R\|_F^2\right)
\end{align*}
    \item Low-rank regression:
\begin{align*}
\argmin_{H,U}&\ \frac{1}{2N} \sum_{(j,i) \in \Omega} \left(Y_{ji} - H_j^\T U \phi_i \right)^2 + \frac{\lambda_1}{2N}  \left( \|H\|_F^2 + \|U\|_F^2 \right)
\end{align*}
    \item Matrix factorization + low-rank regression:
\begin{align*}
\argmin_{L,R,H,U}&\ \frac{1}{2N} \sum_{(j,i) \in \Omega}\left(Y_{ji} - L_j^\T R_i - H_j^\T U\phi_i \right)^2 + \frac{\lambda_1}{2N}  \left( \|H\|_F^2 + \|U\|_F^2\right) + \frac{\lambda_2}{2N}  \left( \|L\|_F^2 +\|R\|_F^2\right)
\end{align*}
    \item Functional regression: 
\begin{align*}
\argmin_{Q}&\ \frac{1}{2N} \sum_{(j,i) \in \Omega}\left(Y_{ji} - B_j^\T Q\phi_i \right)^2 
\end{align*}

    \item Matrix factorization + functional regression:
\begin{align*}
\argmin_{L,R,Q}&\ \frac{1}{2N} \sum_{(j,i) \in \Omega}\left(Y_{ji} - L_j^\T R_i - B_j^\T Q\phi_i \right)^2 + \frac{\lambda_2}{2N}  \left( \|L\|_F^2 +\|R\|_F^2\right)
\end{align*}

    \item Neural Network regression:
\begin{align*}
\argmin_{\psi}&\ \frac{1}{2N} \sum_{(j,i) \in \Omega}\left(Y_{ji} - g_\psi(\phi_i) \right)^2 
\end{align*}
    \item Matrix factorization + neural network regression:
\begin{align*}
\argmin_{L,R,\psi}&\ \frac{1}{2N} \sum_{(j,i) \in \Omega}\left(Y_{ji} - L_j^\T R_i - g_\psi(\phi_i) \right)^2
\end{align*}

\end{itemize}
}
